# Supplementary material for: PDF bias and flavor dependence in TMD distributions
Source: arXiv:2201.07114 source file (2022-07-27)
Supplement: Supplementary file 1 [file SupplementaryMaterials.pdf]

# Supplementary materials

## 1 Comparison to the data

In the following plots, we demonstrate the ratio to the central value of theoretical prediction for all data set studied in the work for all four studied PDFs. Red band is the **EXP**-uncertainty. Light-green band is the **PDF**-uncertainty. The blue band is the combined uncertainty. The filled bullets are included into the fit. Red vertical line shows the expected boundary of the TMD factorization $q_T = 0.25Q$. For a better visual comparison the theory lines are shifted by constant value indicated in percentage at each plot.

*Z-boson production at Tevatron*

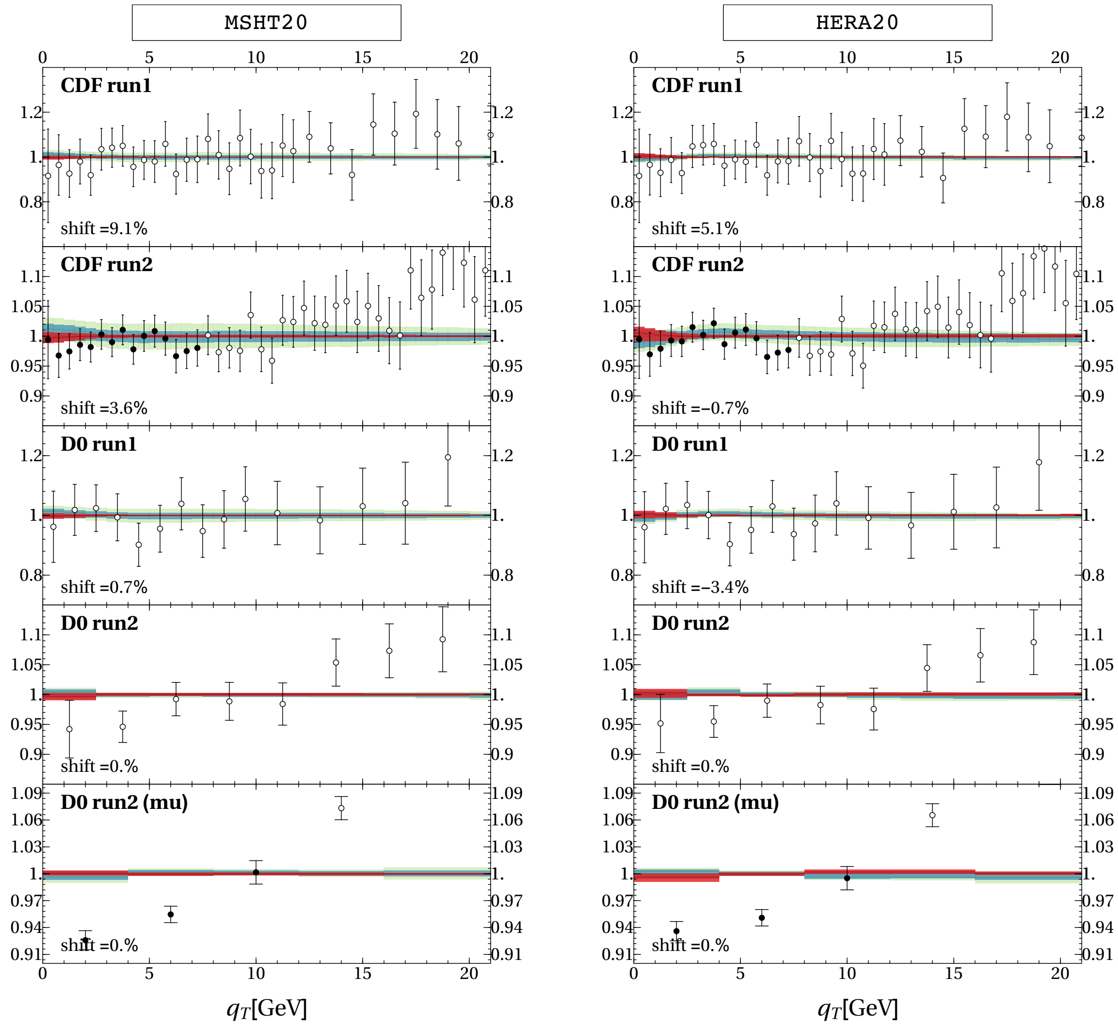

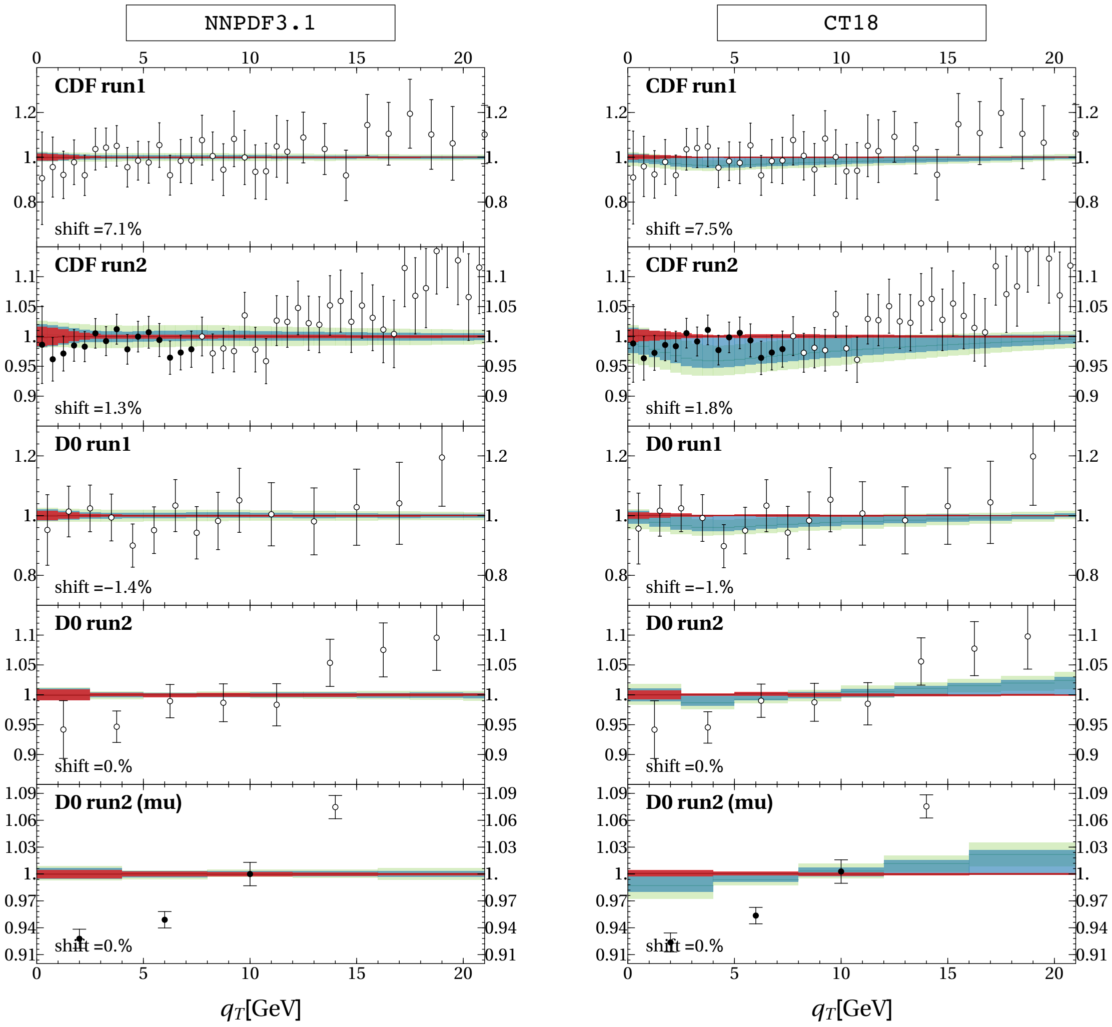


*Z-boson production at 7TeV at ATLAS*

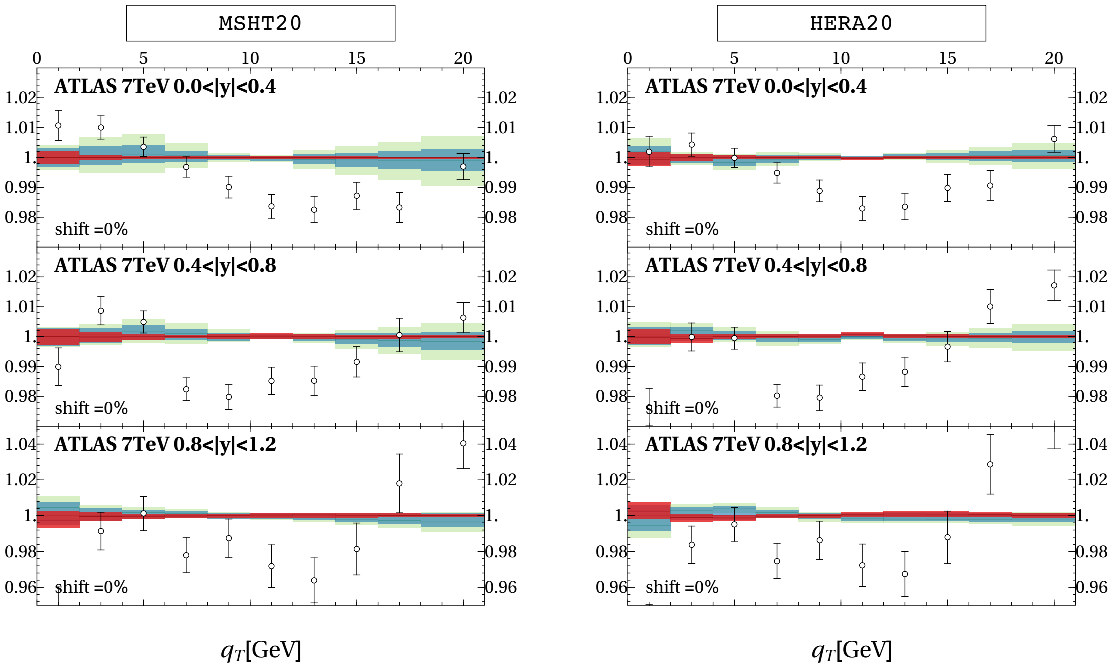

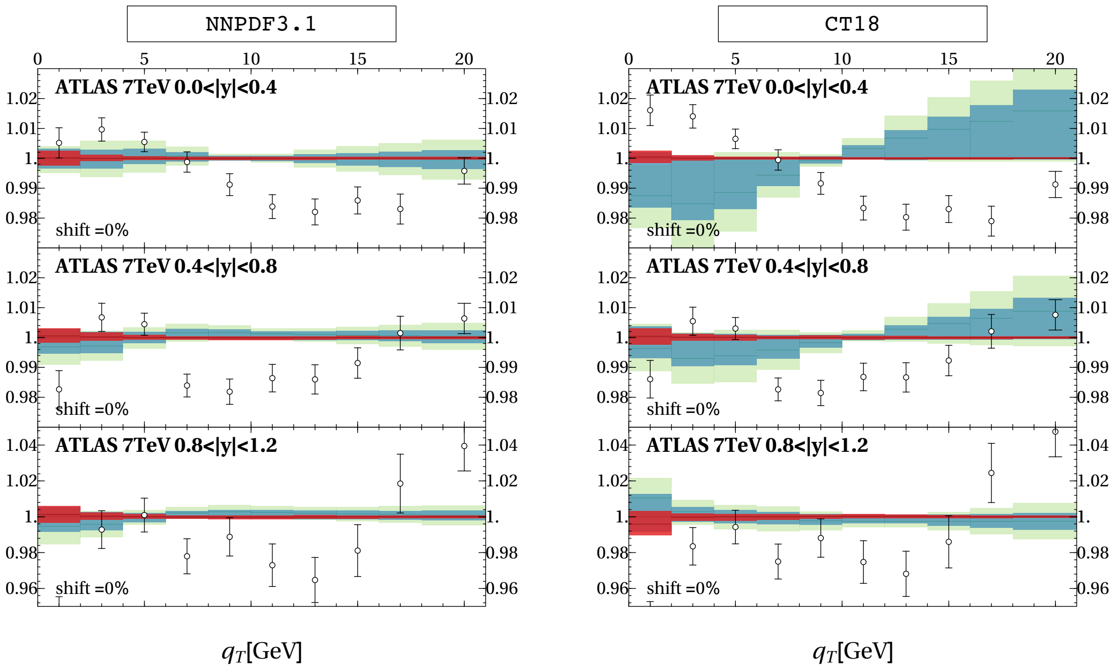


*Z-boson production at 8TeV at ATLAS*

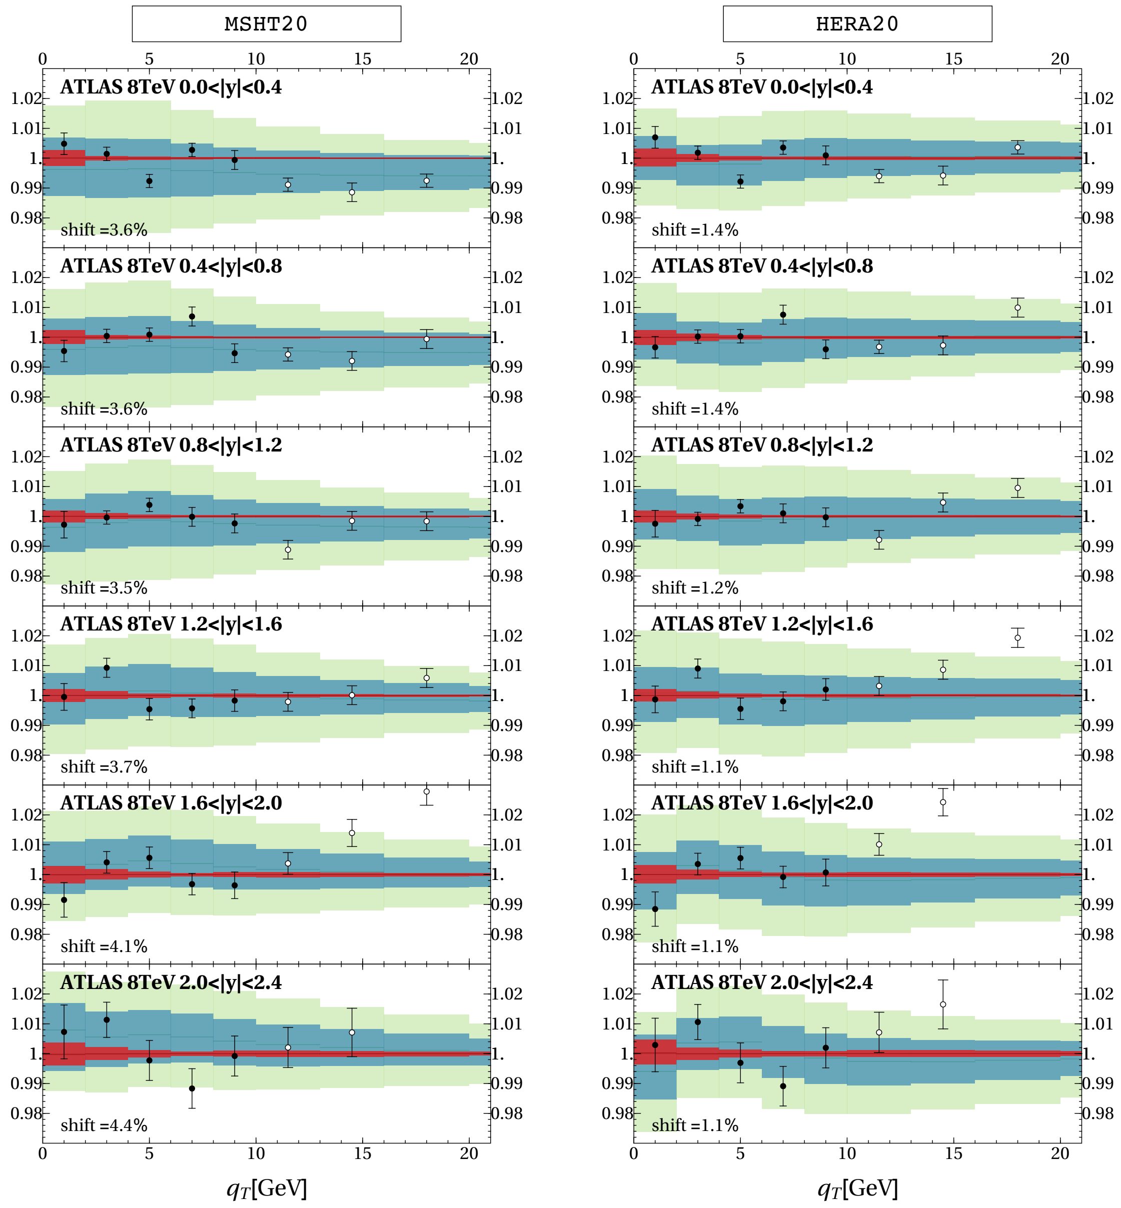

MSHT20
HERA20
ATLAS 8TeV 0.0<|y|<0.4
shift =3.6%
shift =1.4%
ATLAS 8TeV 0.4<|y|<0.8
shift =3.6%
shift =1.4%
ATLAS 8TeV 0.8<|y|<1.2
shift =3.5%
shift =1.2%
ATLAS 8TeV 1.2<|y|<1.6
shift =3.7%
shift =1.1%
ATLAS 8TeV 1.6<|y|<2.0
shift =4.1%
shift =1.1%
ATLAS 8TeV 2.0<|y|<2.4
shift =4.4%
shift =1.1%
$q_T$[GeV]

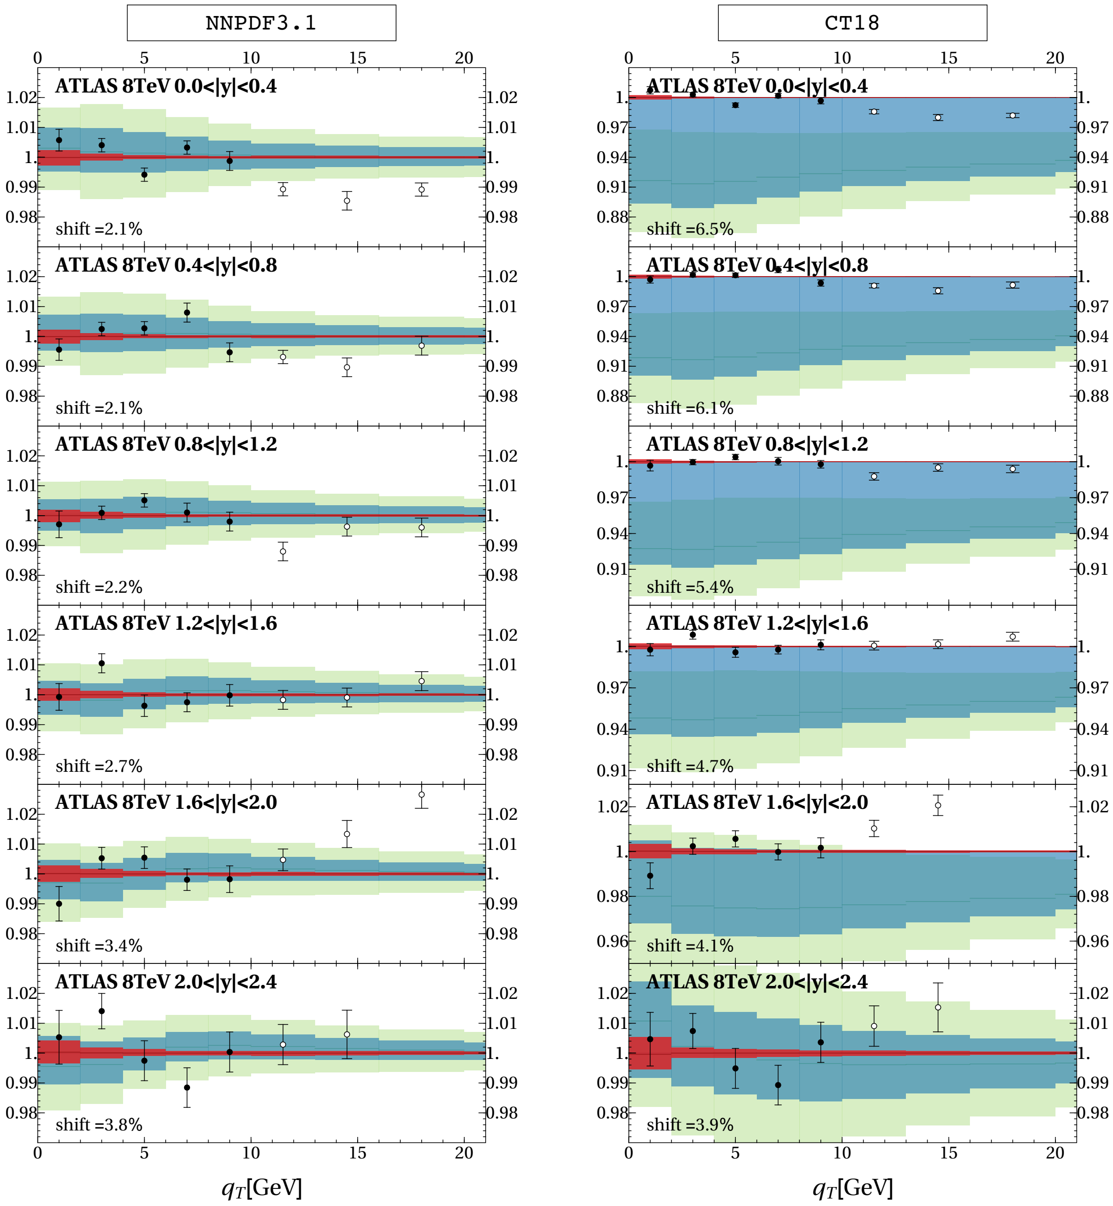


*Z-boson production at LHCb*

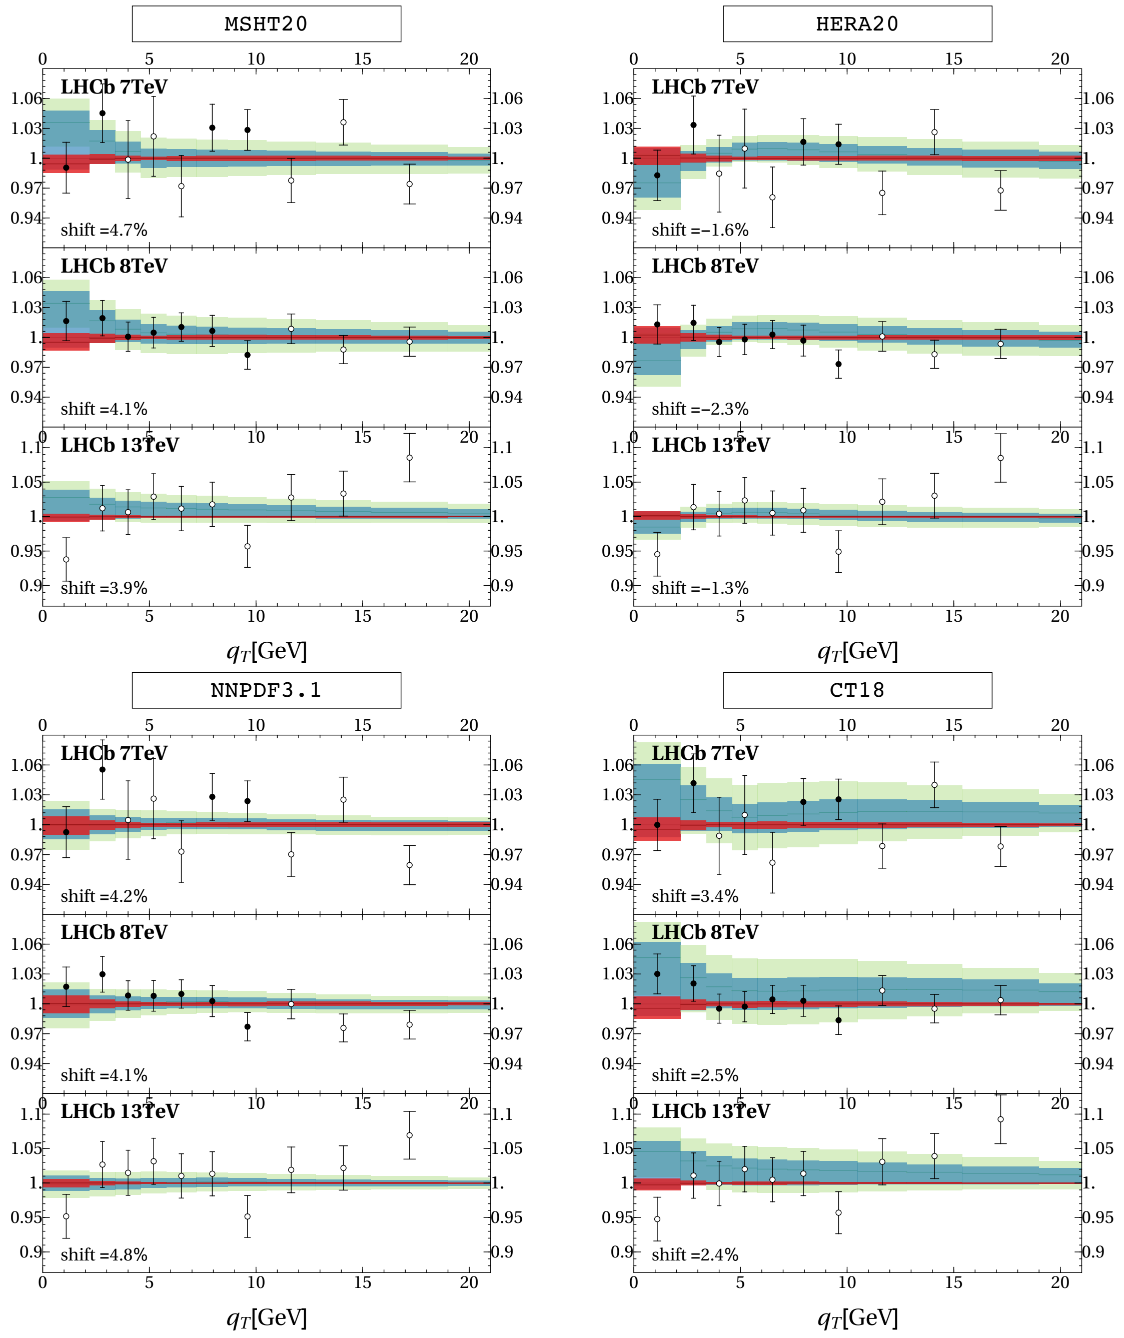


*Z-boson production at 7 and 8 TeV at CMS*

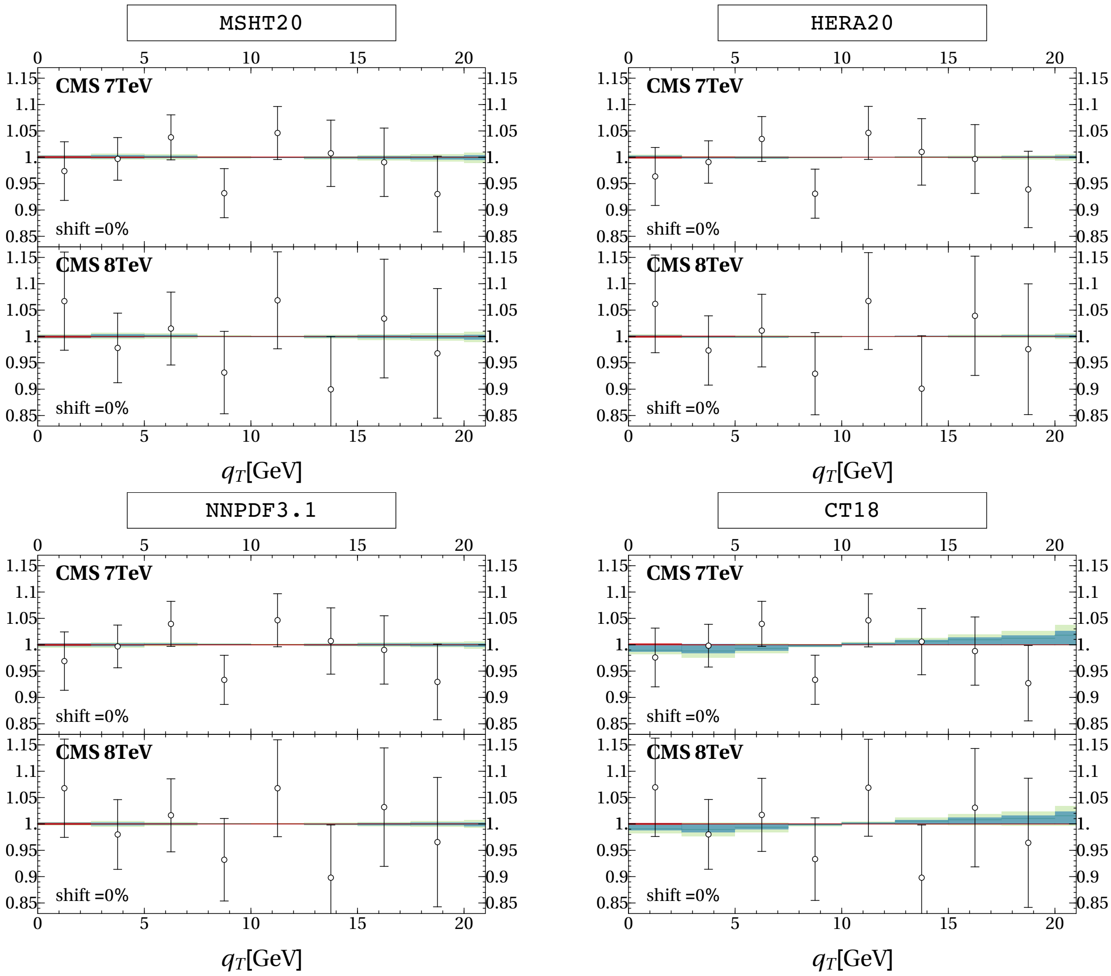


*Z-boson production at 13TeV at CMS*

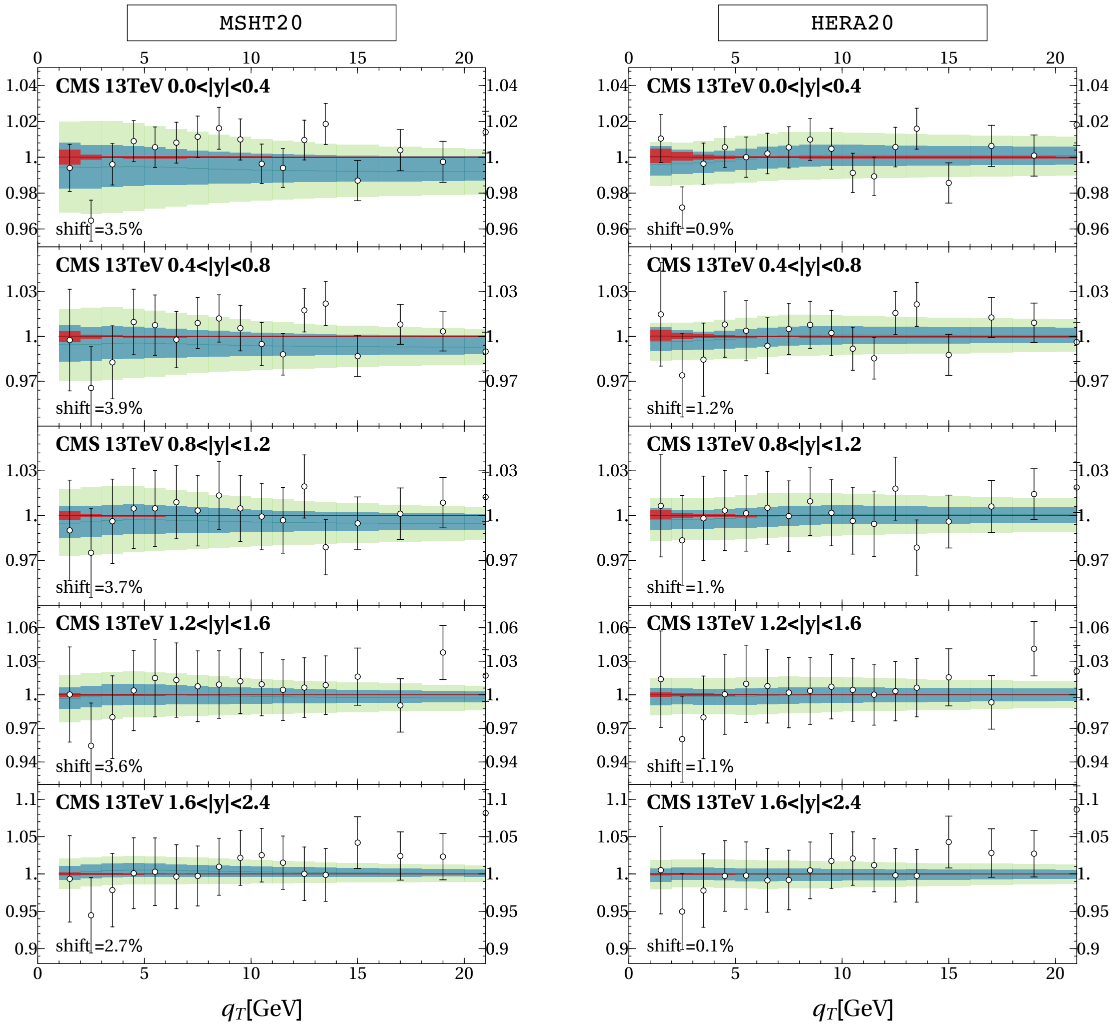
MSHT20
HERA20
CMS 13TeV 0.0<|y|<0.4
shift =3.5%
shift =0.9%
CMS 13TeV 0.4<|y|<0.8
shift =3.9%
shift =1.2%
CMS 13TeV 0.8<|y|<1.2
shift =3.7%
shift =1.%
CMS 13TeV 1.2<|y|<1.6
shift =3.6%
shift =1.1%
CMS 13TeV 1.6<|y|<2.4
shift =2.7%
shift =0.1%
$q_T$[GeV]
$q_T$[GeV]

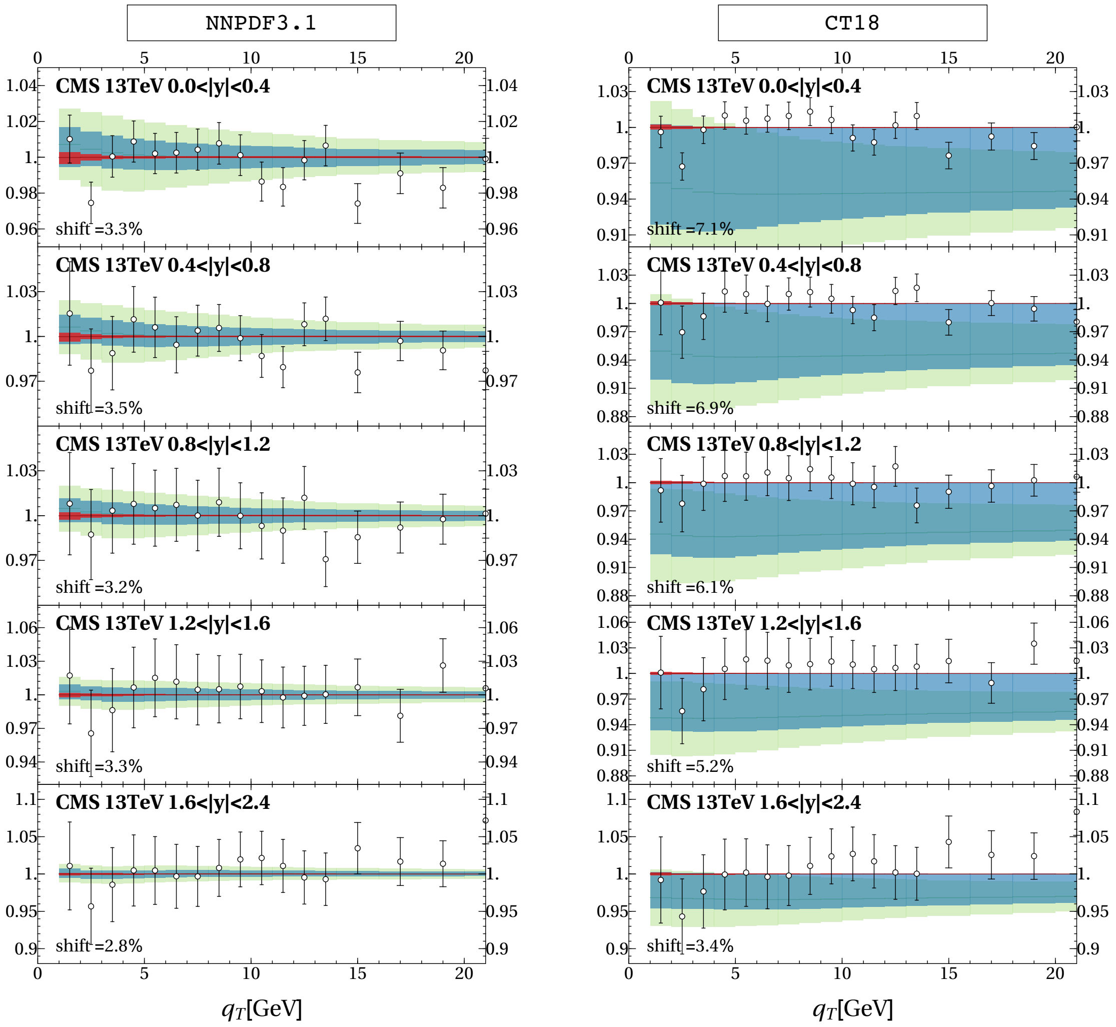


*DY process at E288 with 200GeV beam-energy*

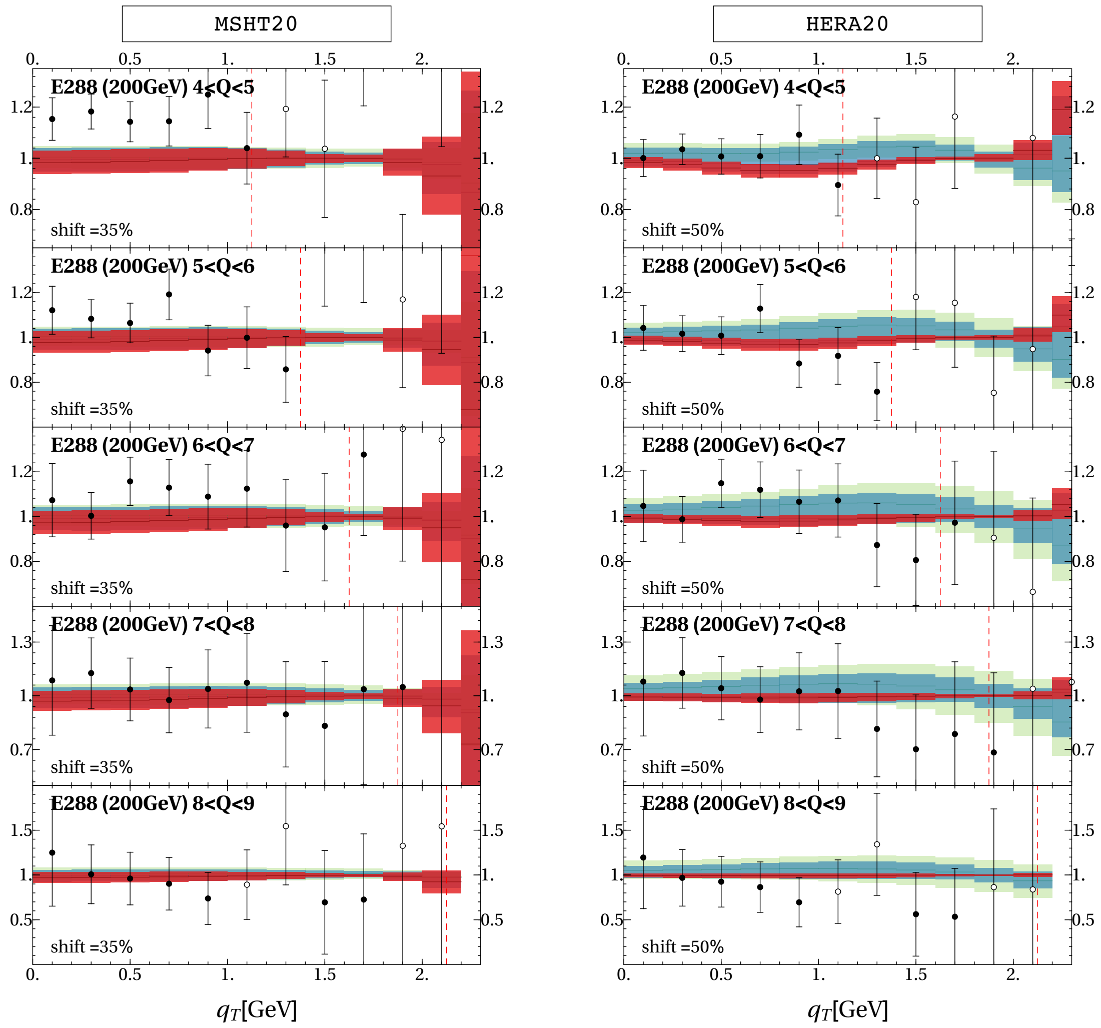
MSHT20
HERA20
E288 (200GeV) 4<Q<5
E288 (200GeV) 5<Q<6
E288 (200GeV) 6<Q<7
E288 (200GeV) 7<Q<8
E288 (200GeV) 8<Q<9
shift =35%
shift =50%
$q_T$[GeV]

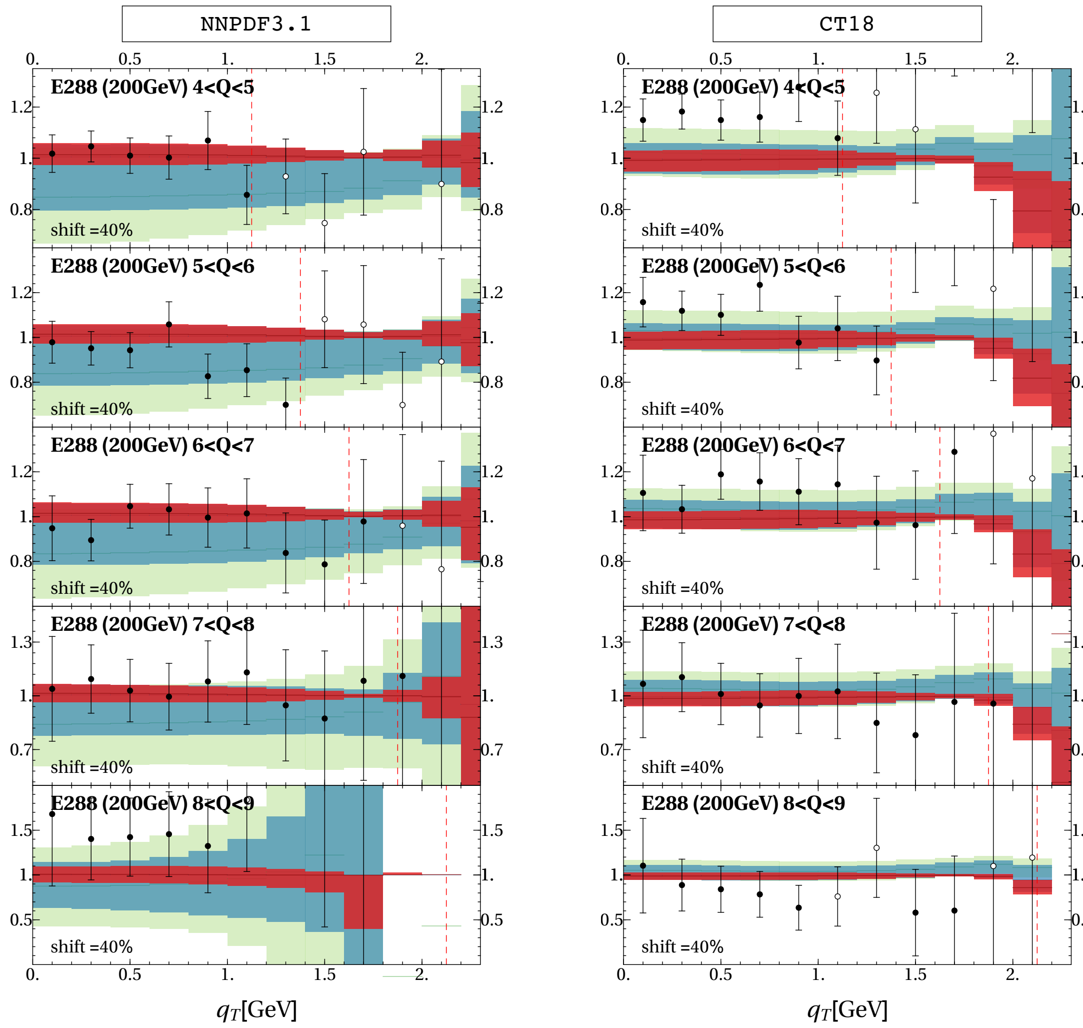


*DY process at E288 with 300GeV beam-energy*

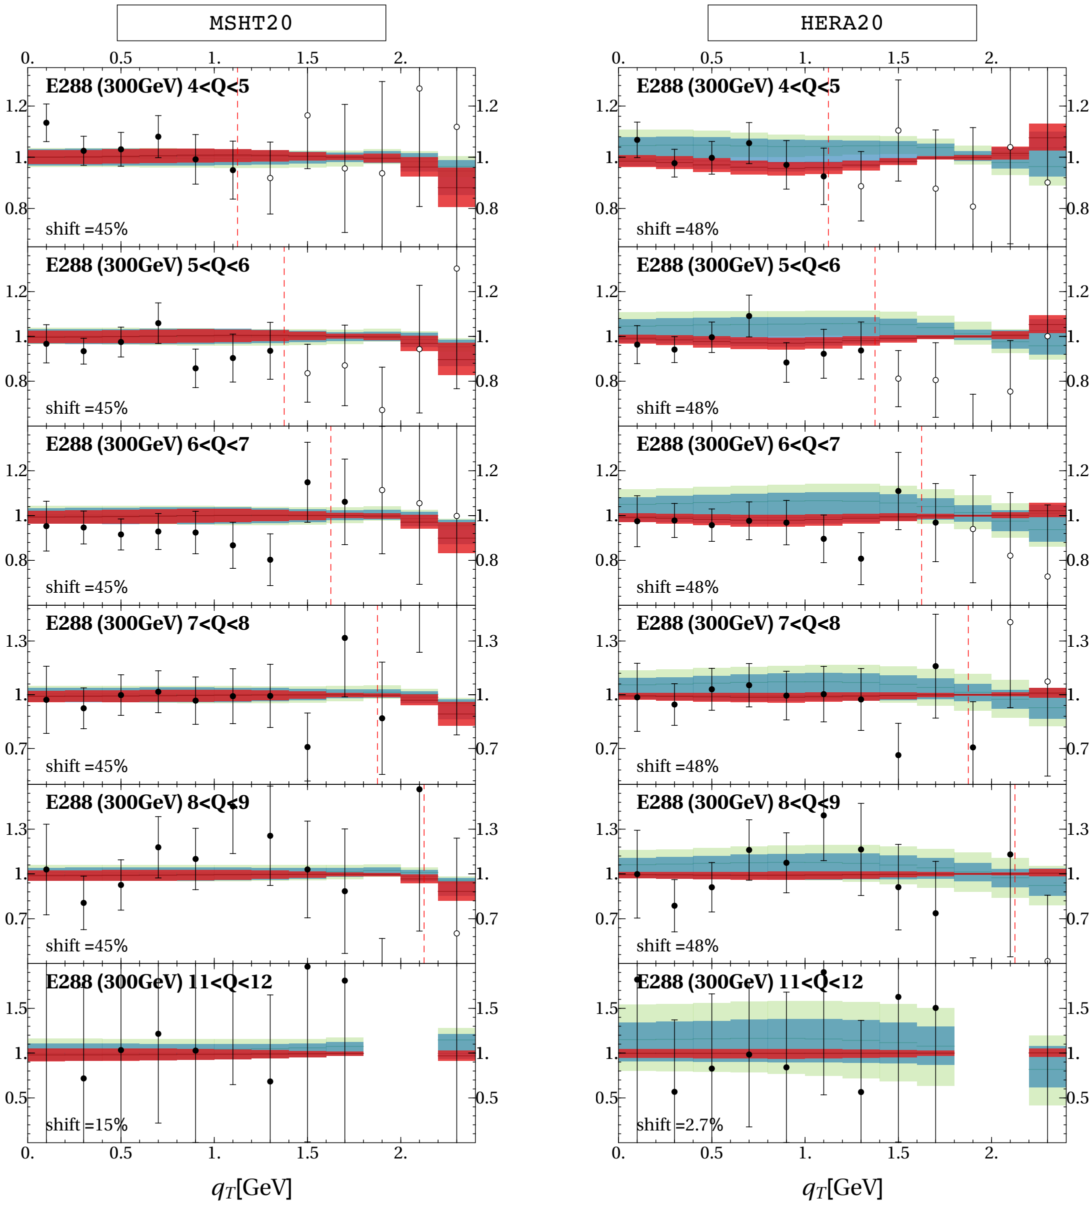
MSHT20
HERA20
E288 (300GeV) 4<Q<5
E288 (300GeV) 5<Q<6
E288 (300GeV) 6<Q<7
E288 (300GeV) 7<Q<8
E288 (300GeV) 8<Q<9
E288 (300GeV) 11<Q<12
shift =45%
shift =15%
shift =48%
shift =2.7%
$q_T$[GeV]

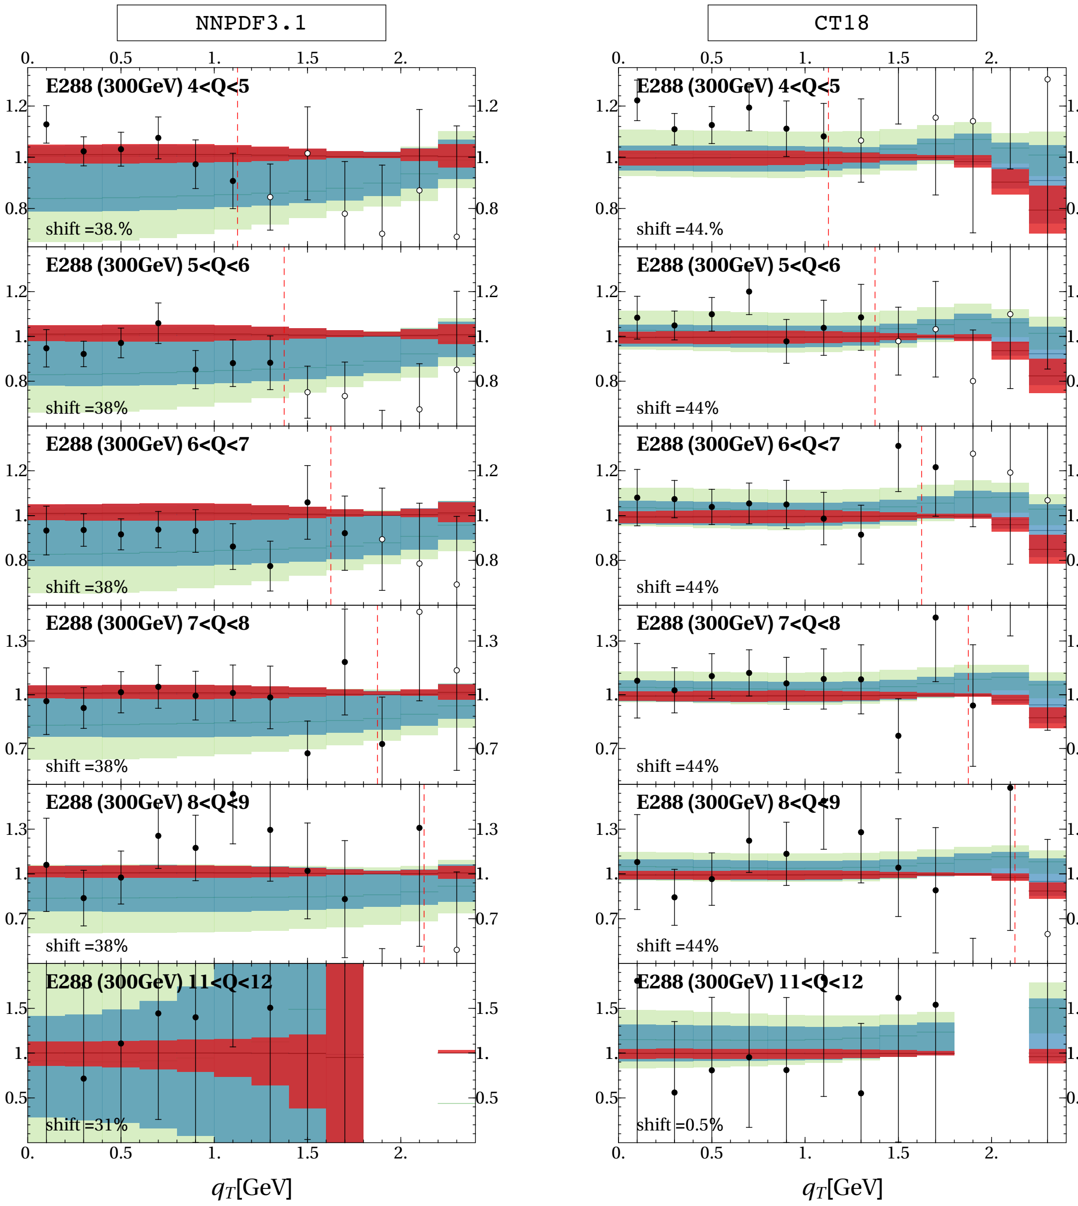


*DY process at E288 with 400GeV beam-energy*

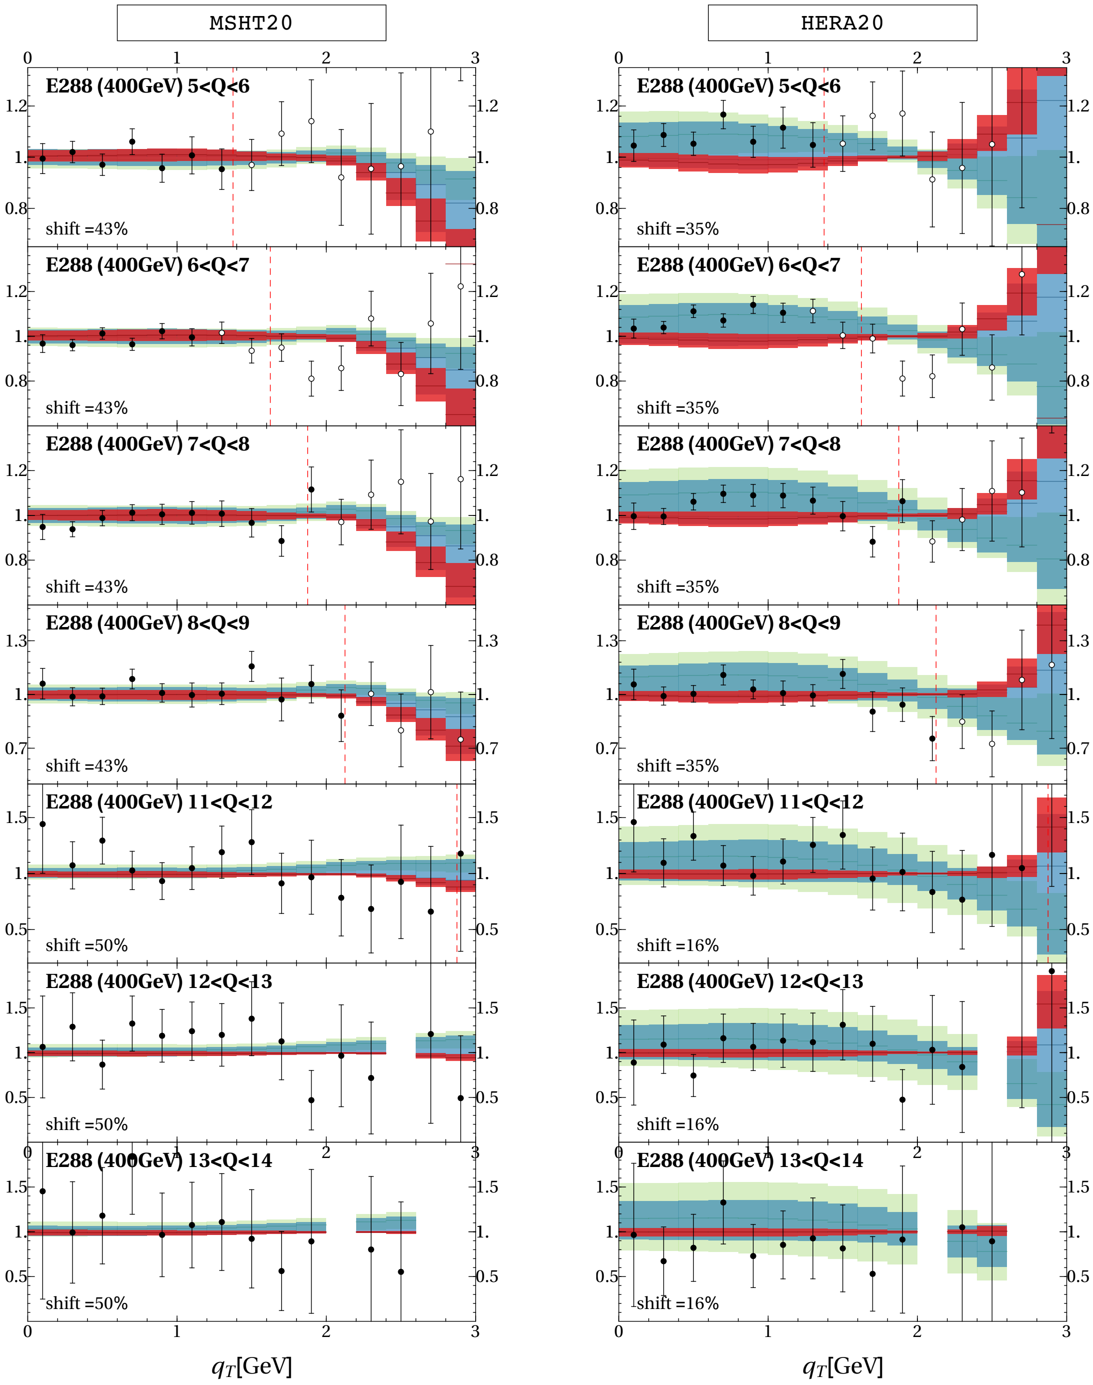

MSHT20
HERA20
E288 (400GeV) 5<Q<6
E288 (400GeV) 6<Q<7
E288 (400GeV) 7<Q<8
E288 (400GeV) 8<Q<9
E288 (400GeV) 11<Q<12
E288 (400GeV) 12<Q<13
E288 (400GeV) 13<Q<14
shift =43%
shift =50%
shift =35%
shift =16%
$q_T$[GeV]

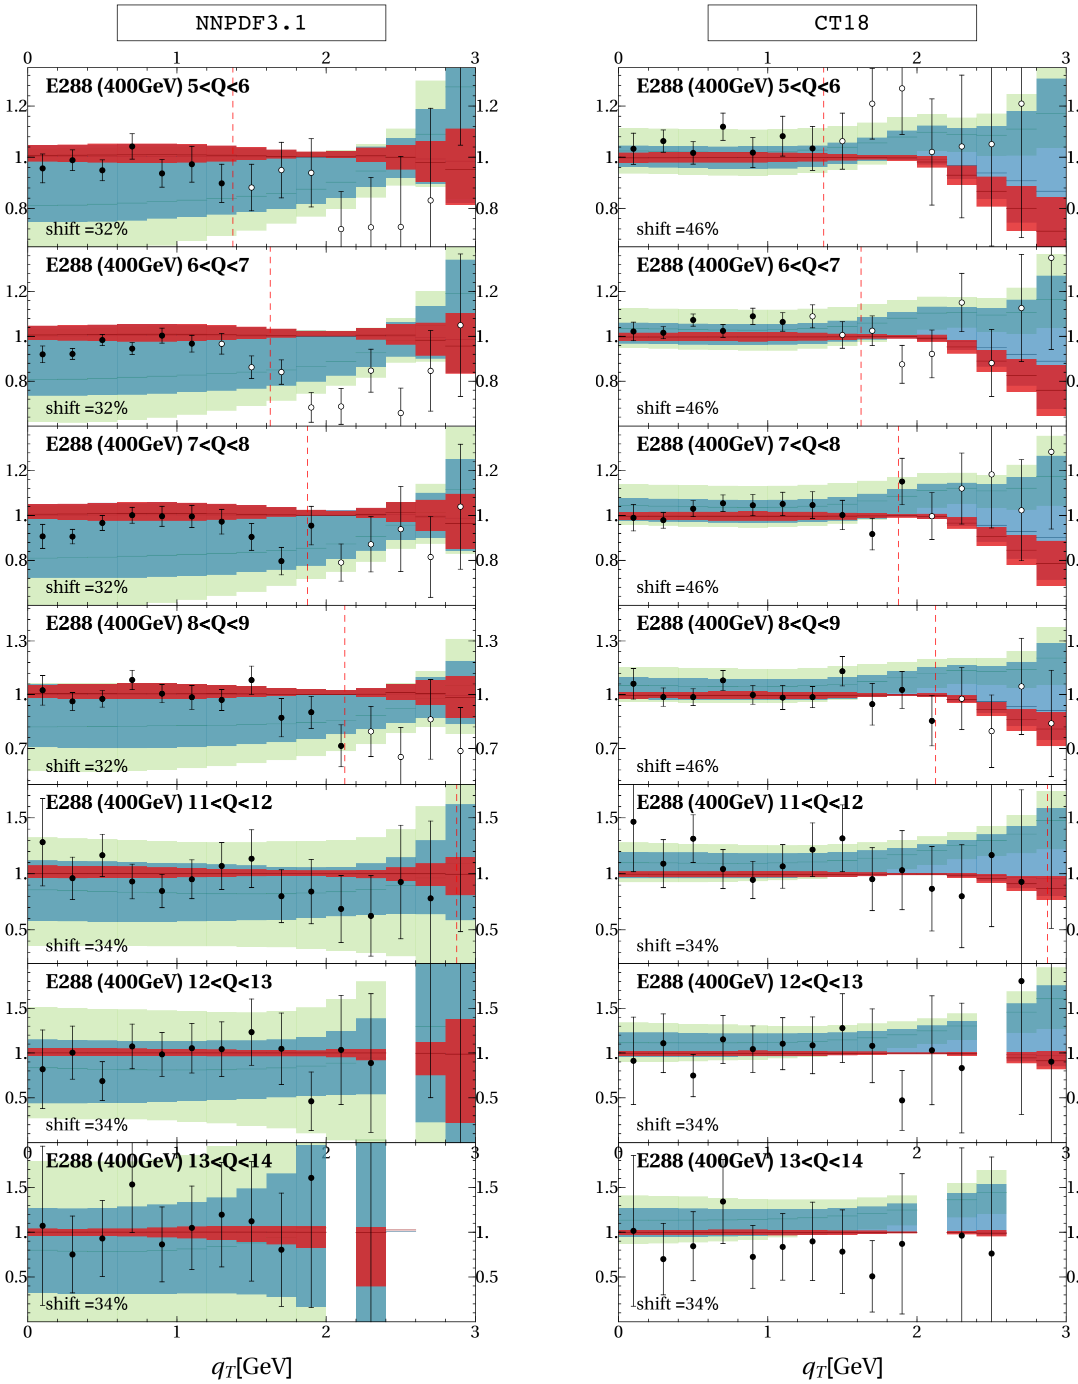


*DY process at E605*

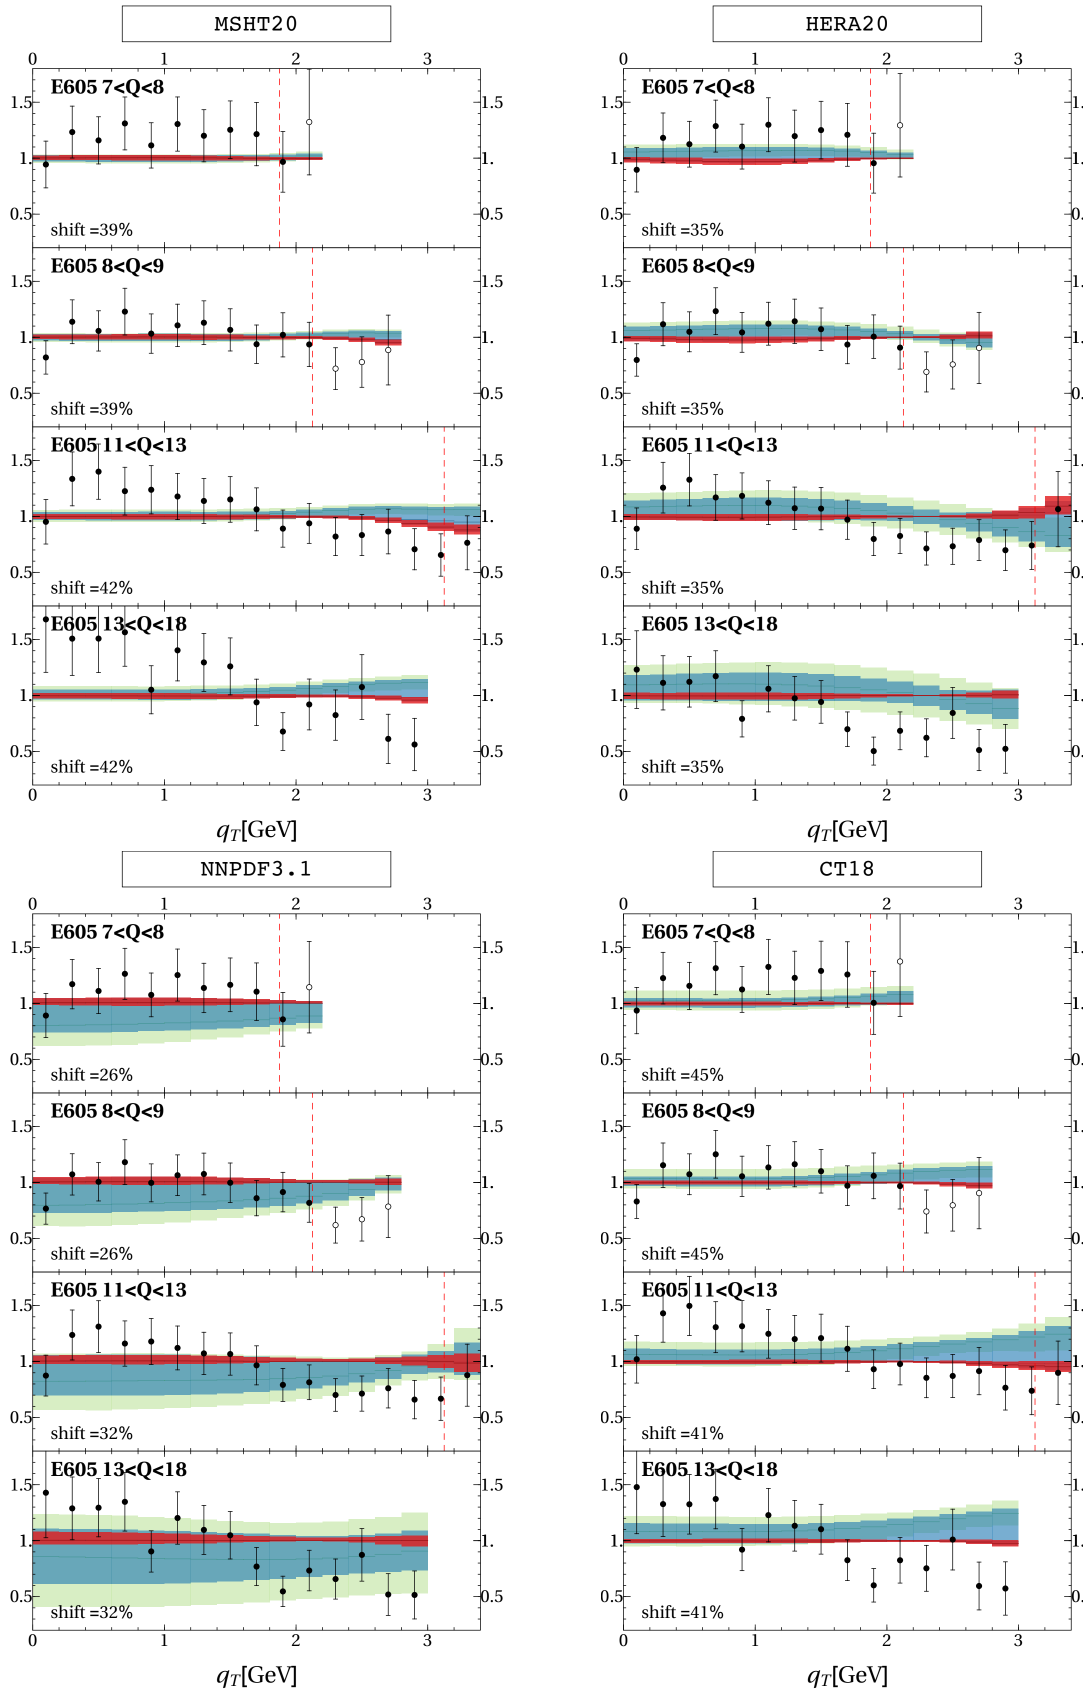


*DY process at E772*

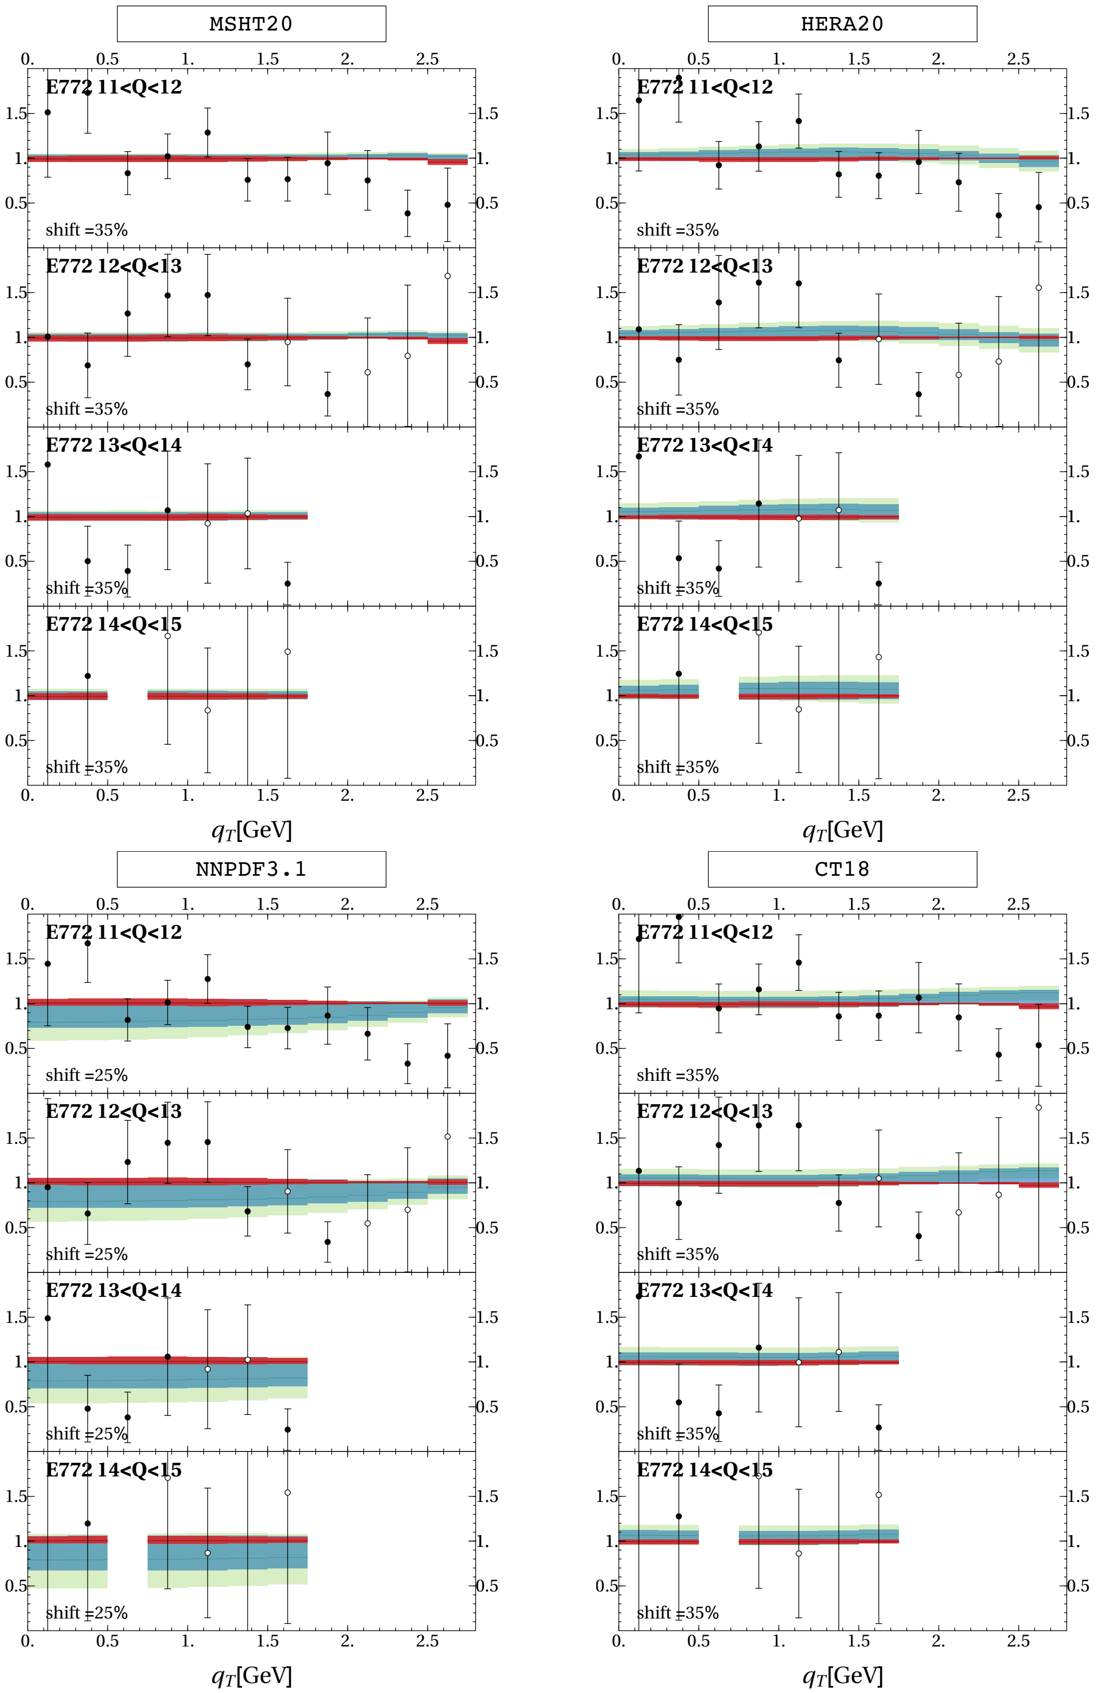
MSHT20
HERA20
NNPDF3.1
CT18
E772 11<Q<12
E772 12<Q<13
E772 13<Q<14
E772 14<Q<15
shift =35%
shift =25%
$q_T$[GeV]

## 2 Extracted TMDPDFs

Shapes of optimal TMD distributions extracted using different PDFs.

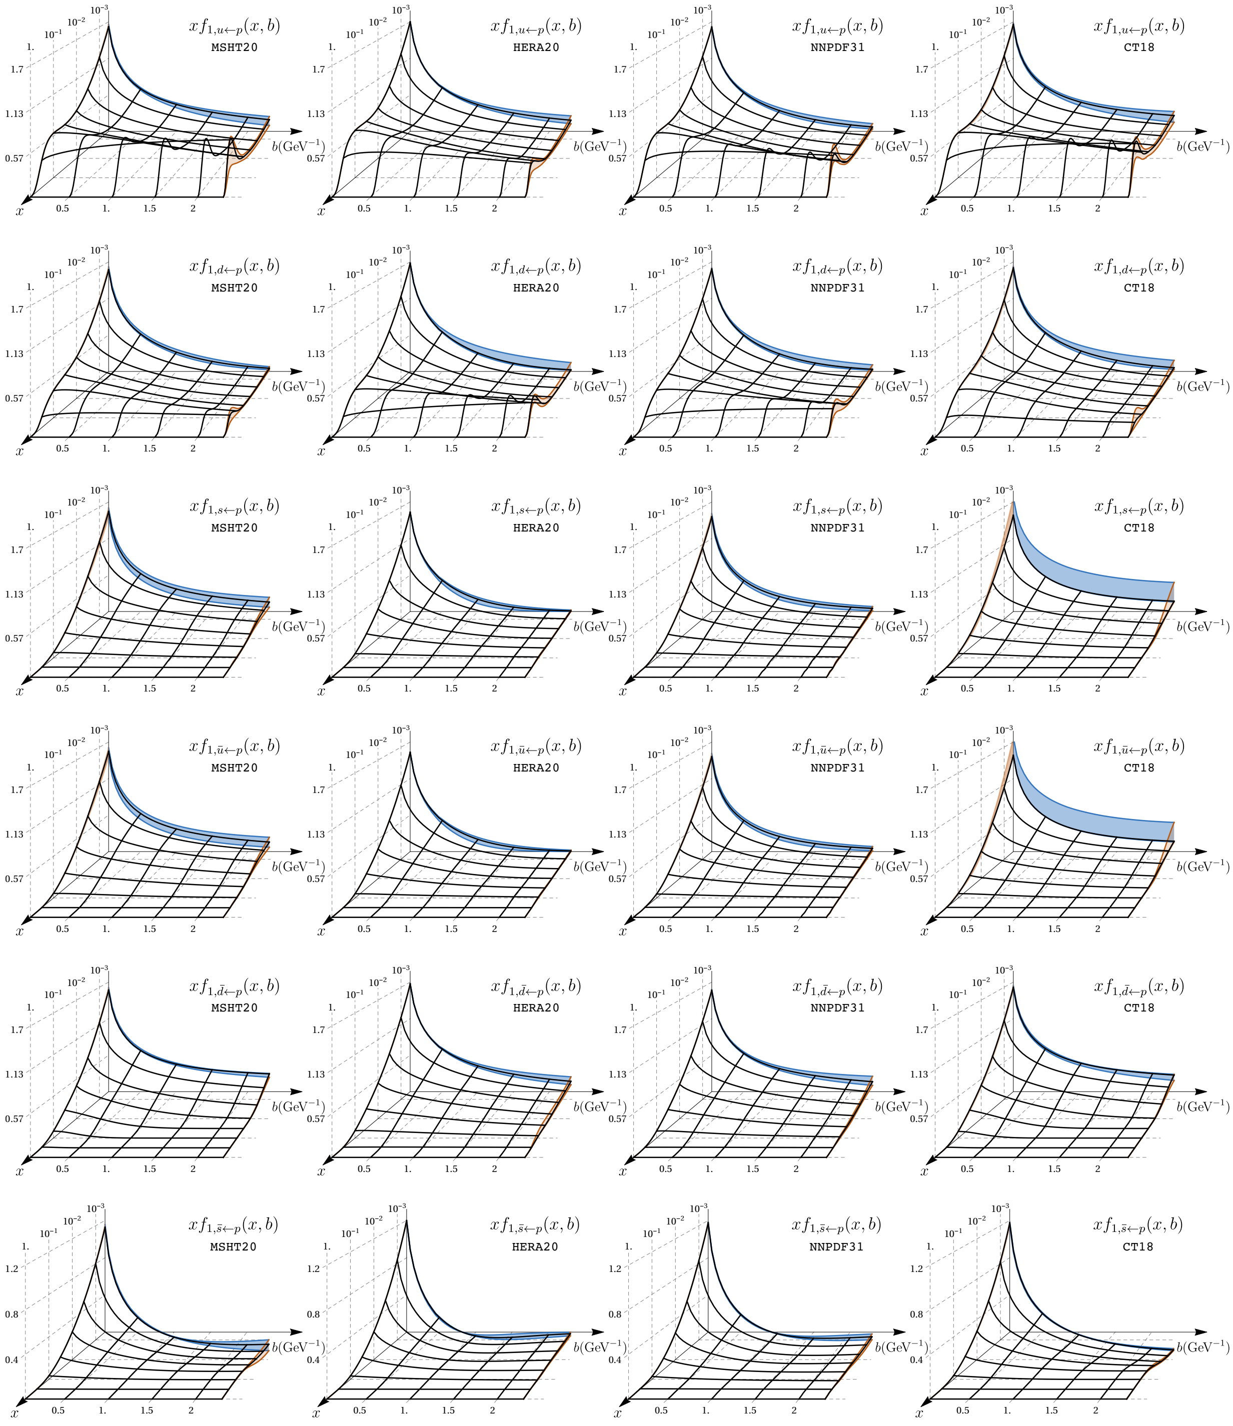


Comparison of uncertainty bands for unpolarized TMDPDFs extracted with different PDFs. The slices of optimal TMDPDF at given values of $b$ or $x$ are presented. For convenience of presentation the plots are weighted with the central TMDPDF value averaged between different PDF cases.

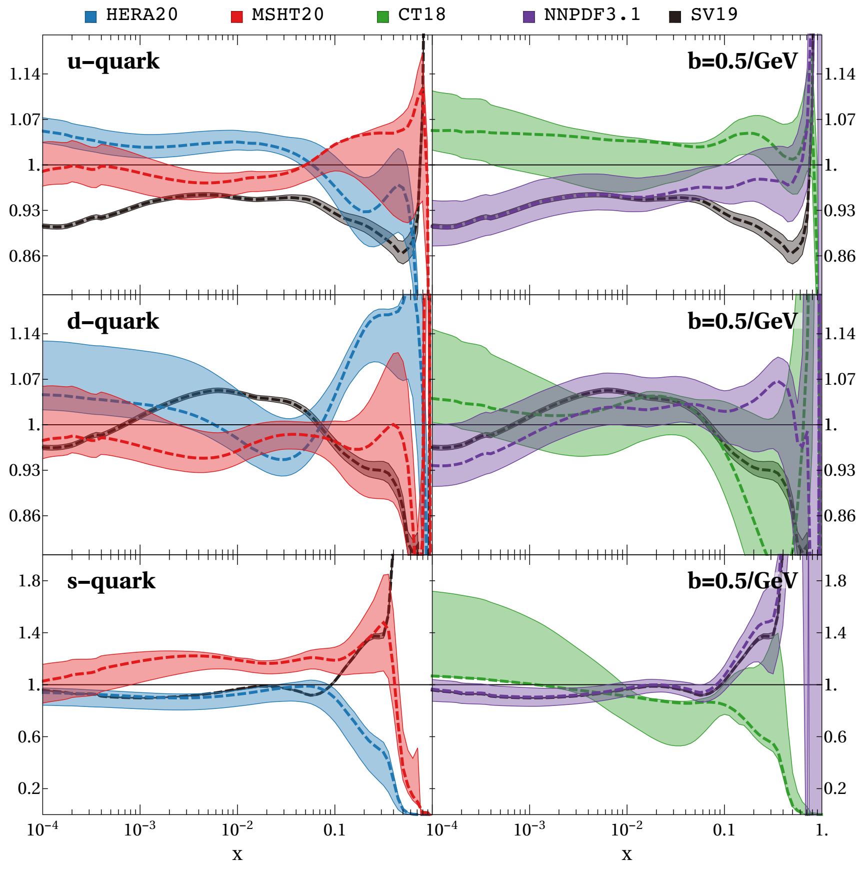

HERA20
MSHT20
CT18
NNPDF3.1
SV19
u–quark
d–quark
s–quark
b=0.5/GeV
x


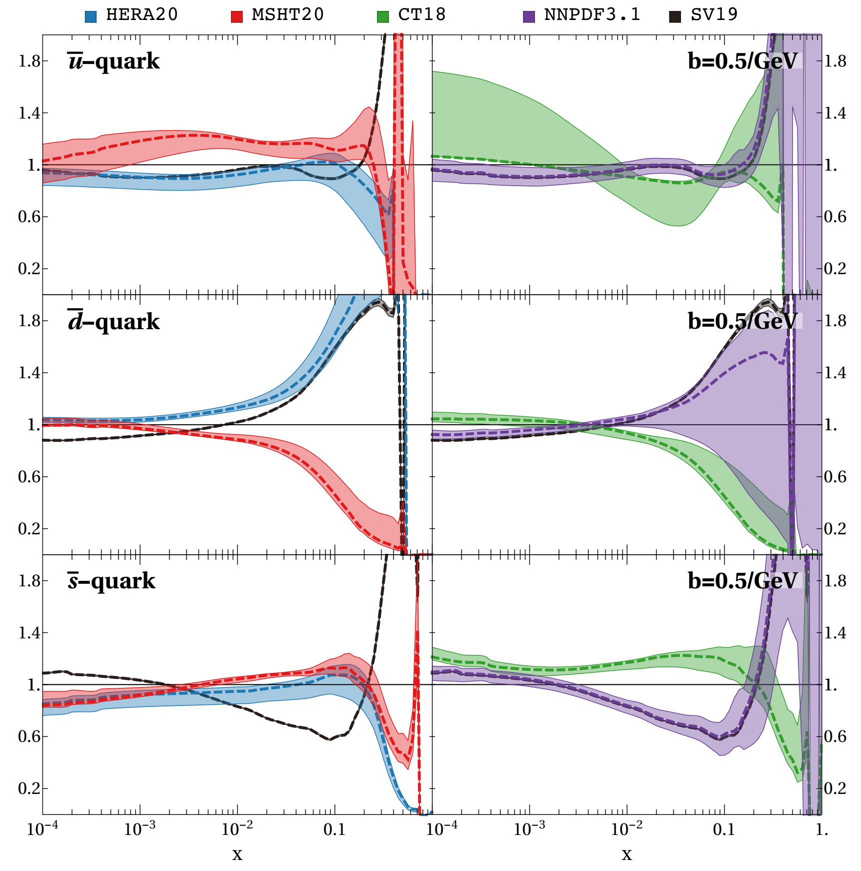

HERA20
MSHT20
CT18
NNPDF3.1
SV19
$\bar{u}$–quark
$\bar{d}$–quark
$\bar{s}$–quark
b=0.5/GeV
x

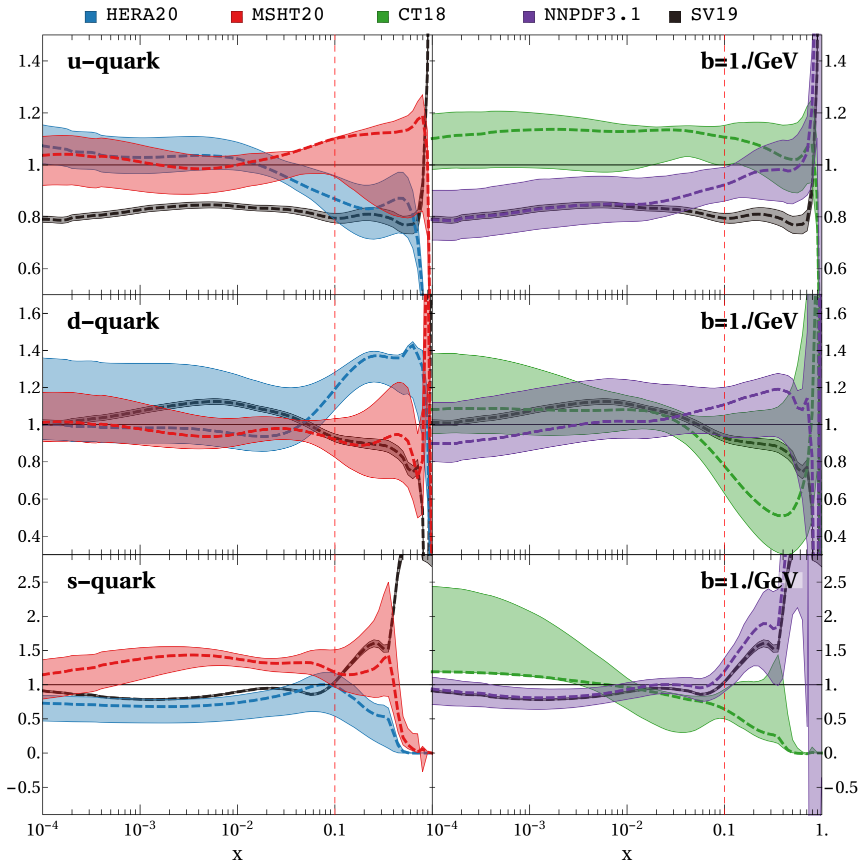

HERA20
MSHT20
CT18
NNPDF3.1
SV19
u–quark
d–quark
s–quark
b=1./GeV
x


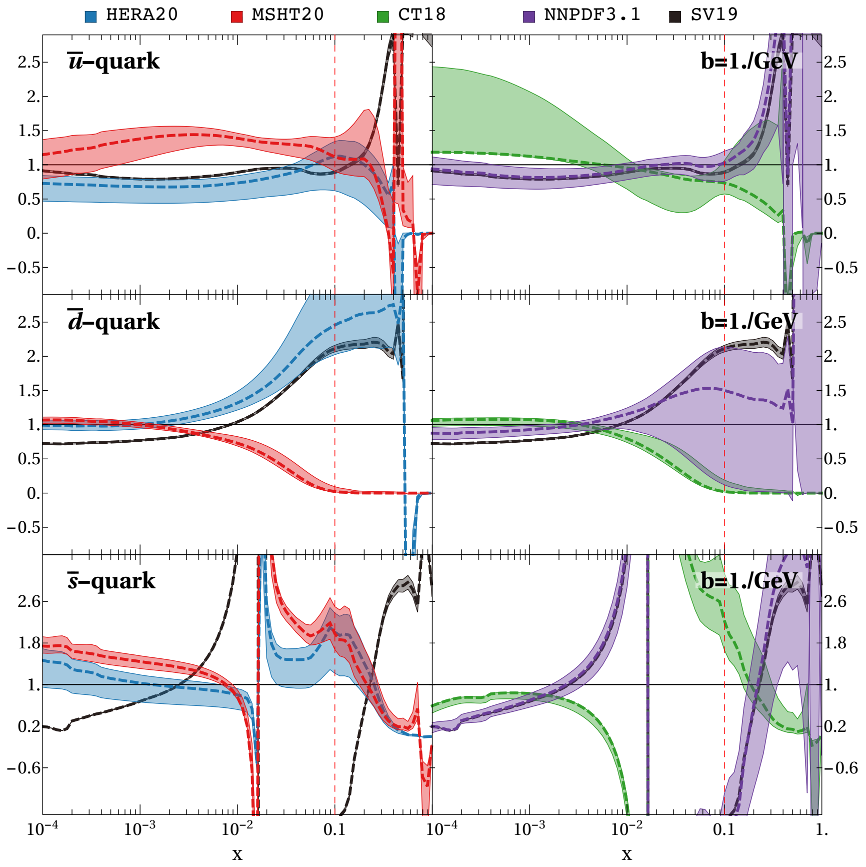

HERA20
MSHT20
CT18
NNPDF3.1
SV19
$\bar{u}$–quark
$\bar{d}$–quark
$\bar{s}$–quark
b=1./GeV
x

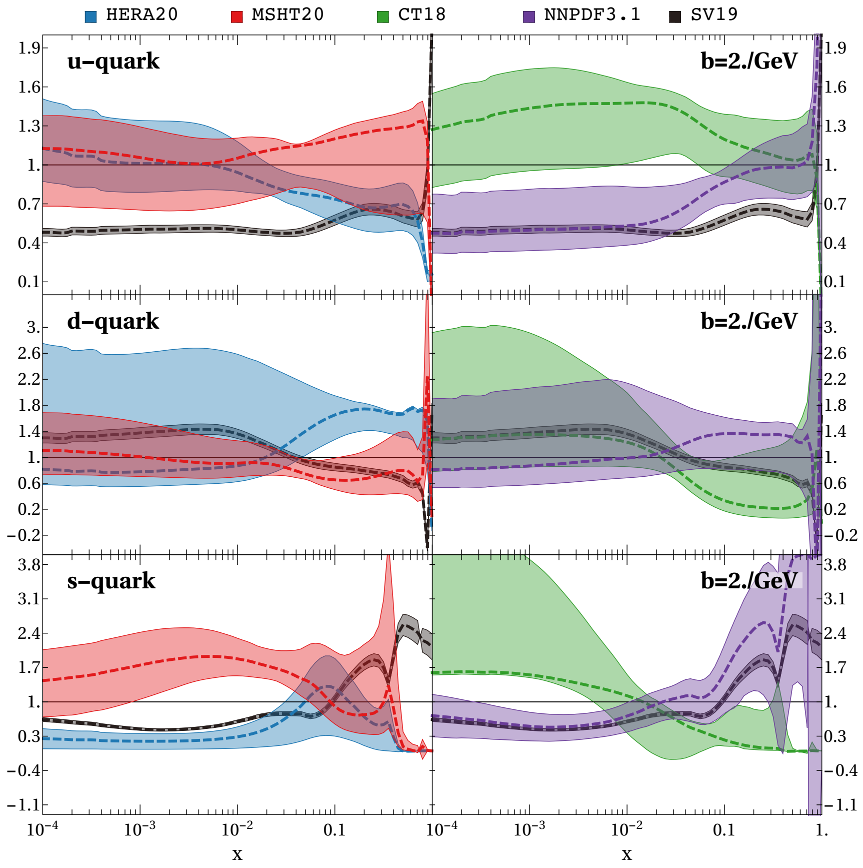
HERA20
MSHT20
CT18
NNPDF3.1
SV19
u−quark
b=2./GeV
d−quark
b=2./GeV
s−quark
b=2./GeV
x
x

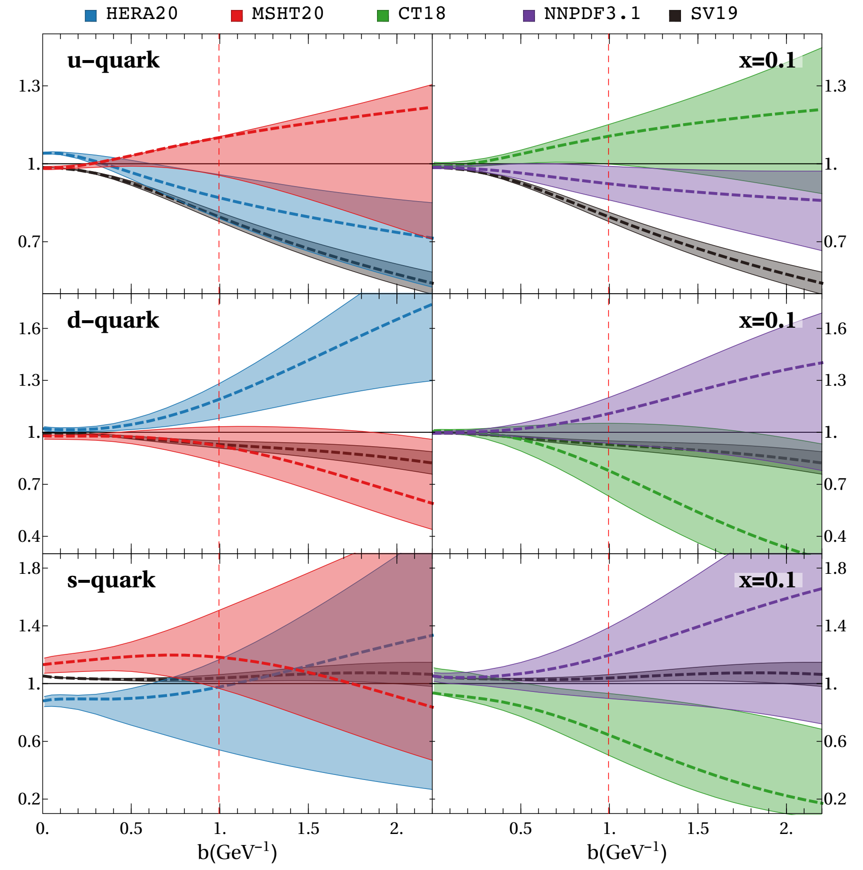
HERA20
MSHT20
CT18
NNPDF3.1
SV19
u−quark
x=0.1
d−quark
x=0.1
s−quark
x=0.1
b(GeV$^{-1}$)
b(GeV$^{-1}$)

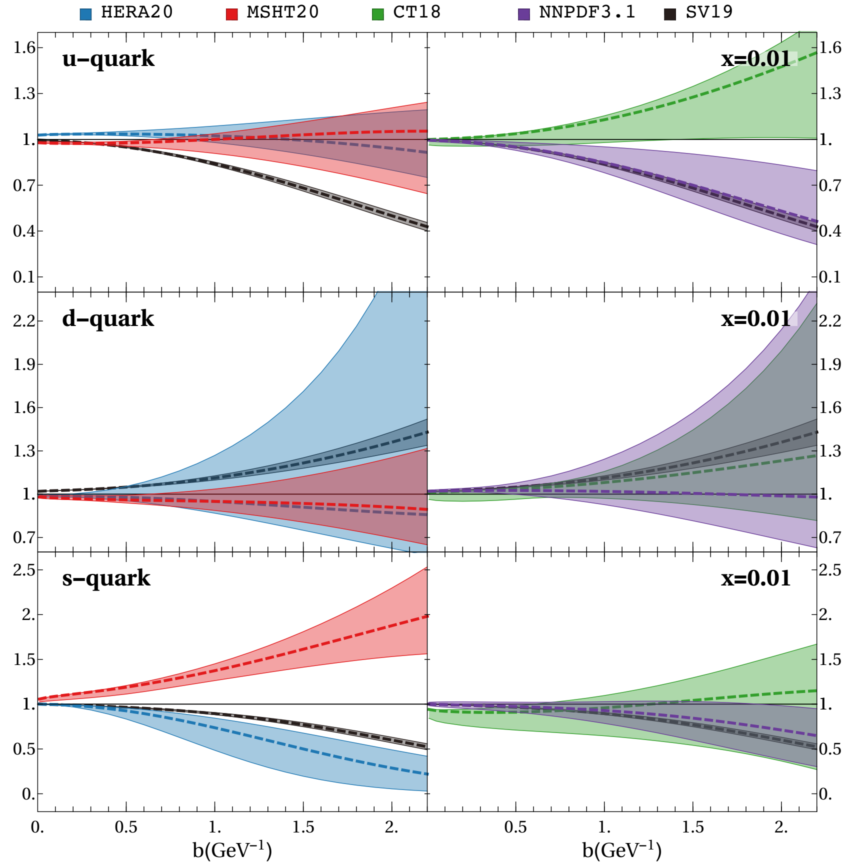
HERA20
MSHT20
CT18
NNPDF3.1
SV19
u–quark
d–quark
s–quark
x=0.01
b(GeV$^{-1}$)

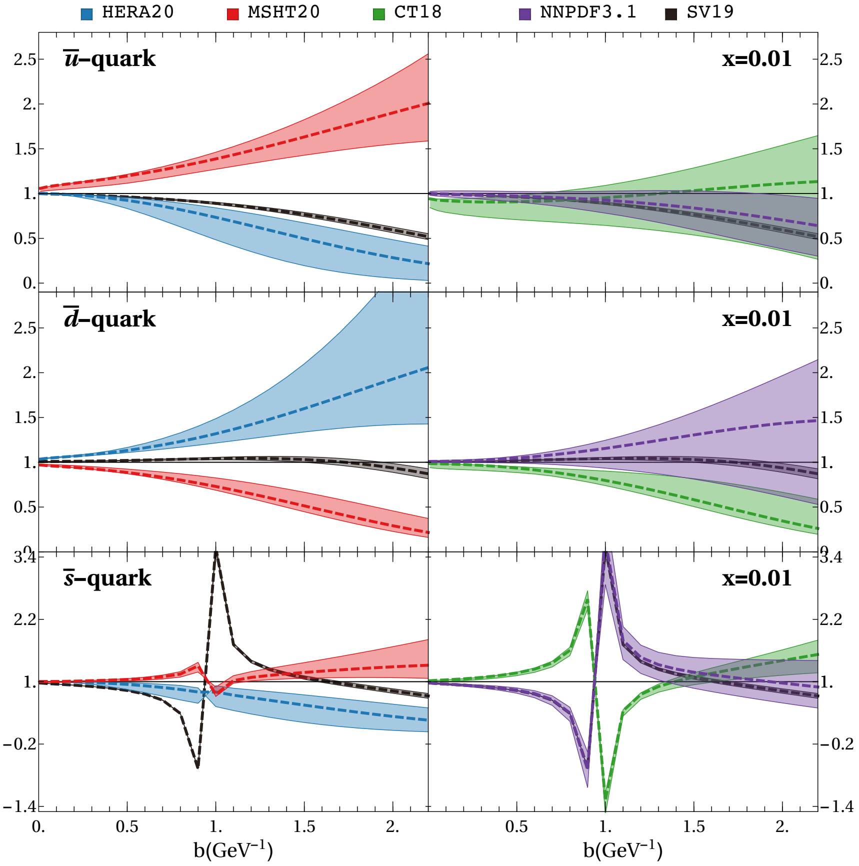
HERA20
MSHT20
CT18
NNPDF3.1
SV19
$\bar{u}$–quark
$\bar{d}$–quark
$\bar{s}$–quark
x=0.01
b(GeV$^{-1}$)

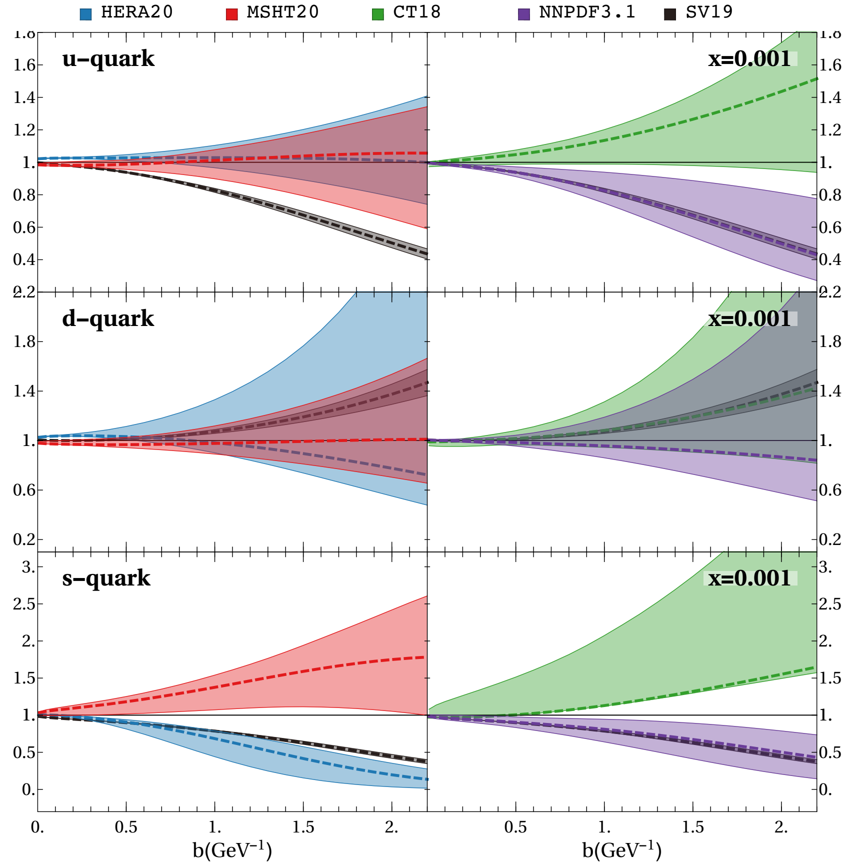
HERA20
MSHT20
CT18
NNPDF3.1
SV19
u–quark
d–quark
s–quark
x=0.001
b(GeV$^{-1}$)

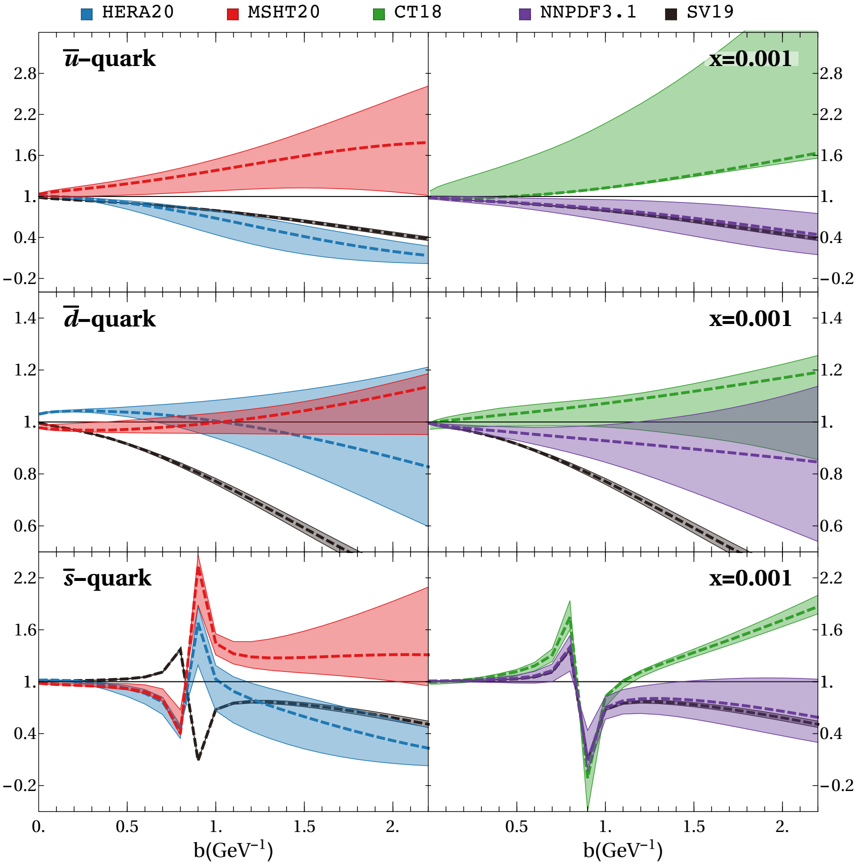
HERA20
MSHT20
CT18
NNPDF3.1
SV19
$\bar{u}$–quark
$\bar{d}$–quark
$\bar{s}$–quark
x=0.001
b(GeV$^{-1}$)

Comparison of uncertainty bands for the ratios of moments of unpolarized TMDPDFs extracted with different PDFs as the function of $b$. The moments are defined as

$$f^{(n)}(b) = \int_{x_{\min}}^{1} dy y^{n-1} f_1(y,b), \tag{2.1}$$

where $x_{\min} = 10^{-5}$.

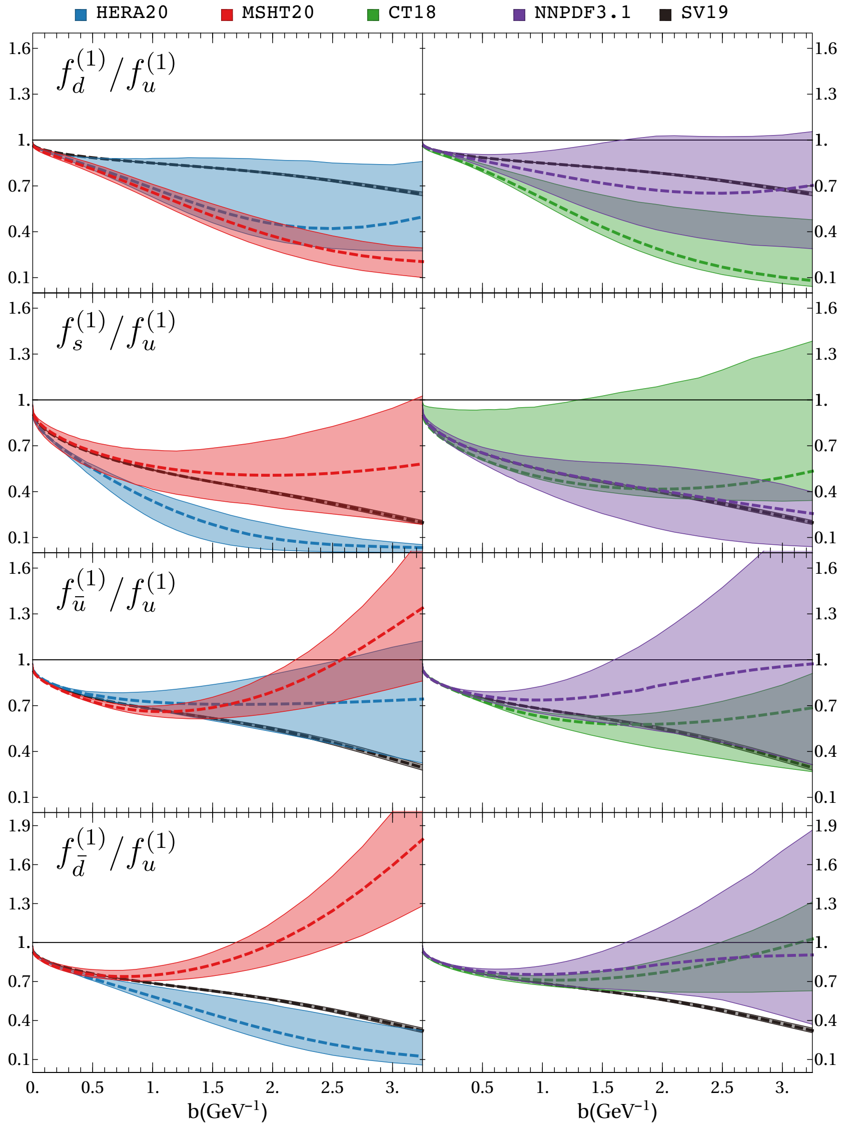

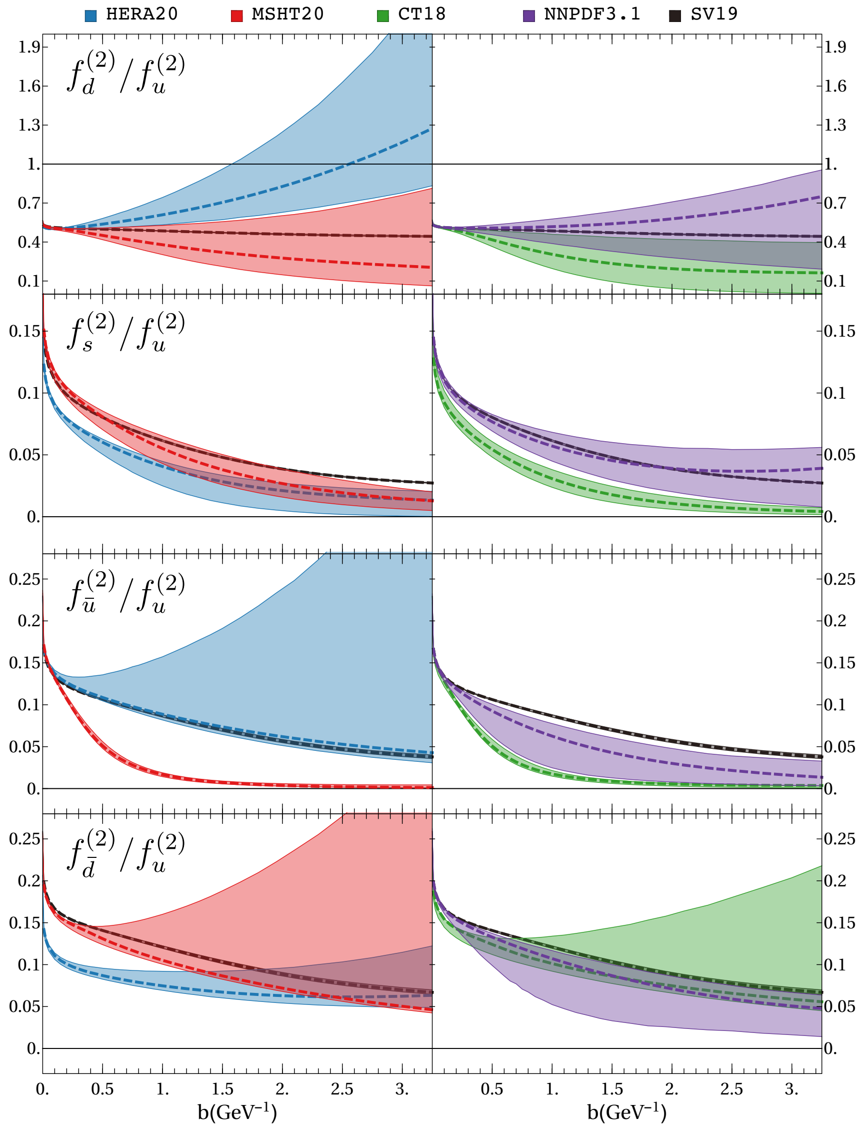
HERA20
MSHT20
CT18
NNPDF3.1
SV19
$f_d^{(2)}/f_u^{(2)}$
$f_s^{(2)}/f_u^{(2)}$
$f_{\bar{u}}^{(2)}/f_u^{(2)}$
$f_{\bar{d}}^{(2)}/f_u^{(2)}$
b(GeV$^{-1}$)
b(GeV$^{-1}$)

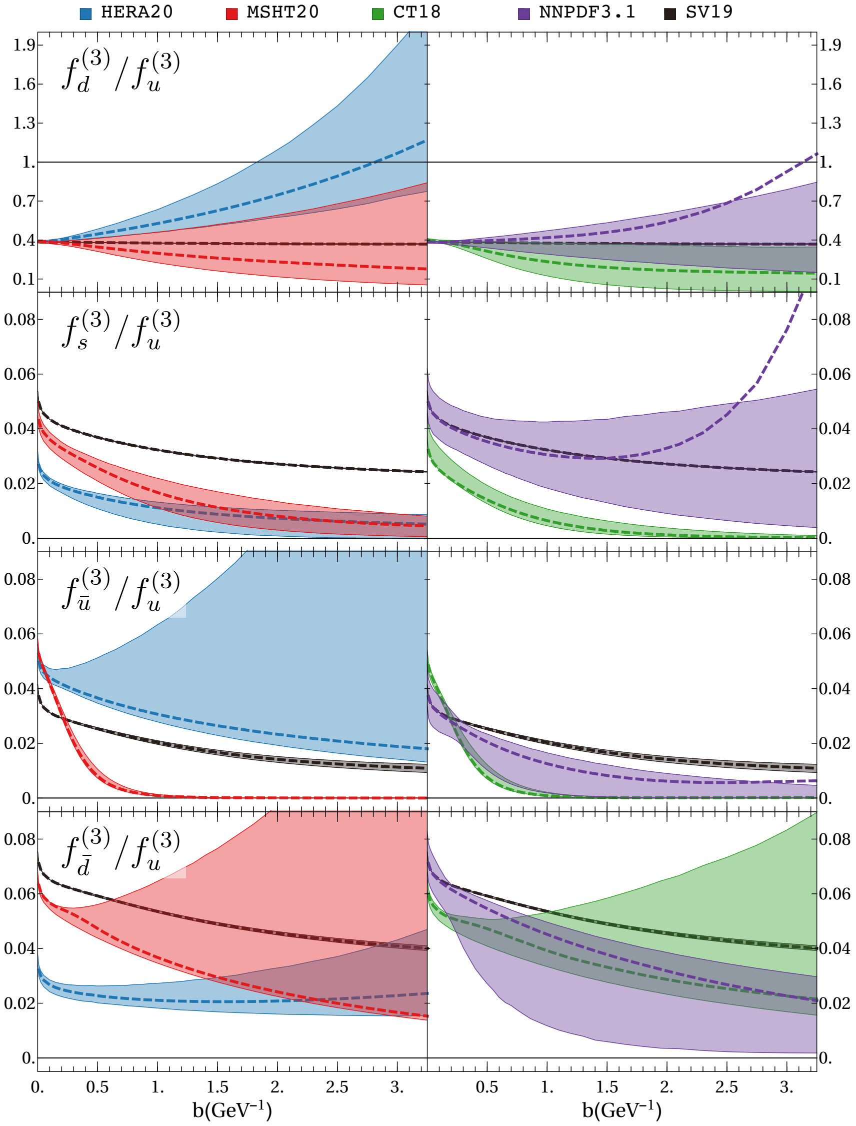
HERA20
MSHT20
CT18
NNPDF3.1
SV19
$f_d^{(3)}/f_u^{(3)}$
$f_s^{(3)}/f_u^{(3)}$
$f_{\bar{u}}^{(3)}/f_u^{(3)}$
$f_{\bar{d}}^{(3)}/f_u^{(3)}$
b(GeV$^{-1}$)
b(GeV$^{-1}$)
